# Supplementary material for: Precision phenomenology of the PDF-BSM interplay
Source: arXiv:2503.02827 source file (2025-03-04)
Supplement: Supplementary file 2 [file tab_chi2_w8.tex]

\begin{table}[t]
        \tiny
        \centering
        \begin{tabular}{lc|c|c|c|c|c|}
                \toprule
       & & \multicolumn{2}{c}{SM} & \multicolumn{2}{c}{$W=8\cdot 10^{-5}$}\\
          \midrule
       Dataset  & $n_{\rm dat}$ & $\chi^2$ &  $n_\sigma$ & $\chi^2$ & $n_\sigma$ \\
          \midrule
 NMC $F^d_2/F^p_2$         & 121 & 0.90 & -0.78 & 0.94 &-0.47 \\
 NMC $\sigma^{\rm NC,p}$ & 204 & 0.93 & -0.71 & 0.93 &-0.71 \\
 SLAC $F^p_2$                   & 33 & 0.52 & -1.95 & 0.55 & -1.83 \\
SLAC $F^d_2$                   & 34 & 1.12 & +0.49 &  1.12 & +0.49 \\
BCDMS $F^p_2$                & 333 & 1.04 & +0.51 &1.03 &+0.39 \\
BCDMS $F^d_2$                & 248 & 0.93 & -0.78 & 0.93 &-0.78 \\
CHORUS $\sigma^\nu_{\rm CC}$ & 416 & 0.98 &-0.28&0.98 &-0.28 \\
CHORUS $\sigma^{\bar\nu}_{\rm CC}$& 416 & 0.95 &-0.72&0.95 &-0.72 \\
NuTeV $\sigma^\nu_{\rm CC}$ (dimuon) & 39 & 0.85 &-0.66& 0.87 &-0.57 \\
NuTeV $\sigma^{\bar\nu}_{\rm CC}$ (dimuon) & 37 & 0.48&-2.23& 0.59&-1.76 \\
                    \midrule
HERA I+II $\sigma^p_{\rm NC} e^-$ & 159 & 1.01&+0.09& 1.02&+0.18 \\
HERA I+II $\sigma^p_{\rm NC} e^+$ (460 GeV) & 204 &0.95&-0.51& 0.95&-0.51 \\
HERA I+II $\sigma^p_{\rm NC} e^+$ (575 GeV) & 254 &1.12 &+1.35&1.12 &+1.35 \\
HERA I+II $\sigma^p_{\rm NC} e^+$ (820 GeV) & 70 &0.89 &-0.65&0.90 &-0.59 \\
HERA I+II $\sigma^p_{\rm NC} e^+$ (920 GeV) & 377 & 0.94&-0.82&0.95 &-0.69 \\
          HERA I+II $\sigma^p_{\rm CC} e^+$ & 42 & 1.22&+1.01&1.22 &+1.01 \\
          HERA I+II $\sigma^p_{\rm CC} e^+$ & 39 & 1.06 &+0.26&1.03 &+0.13\\
          HERA I+II $\sigma^c_{\rm NC}$    & 37 & 0.83 &-0.73&0.84 &-0.69 \\
         HERA I+II $\sigma^b_{\rm NC}$     & 26 & 1.15 &+0.54&1.15&+0.54 \\
                \midrule
                \textbf{Total DIS} & \textbf{3089} & \textbf{0.98} &-0.79&\textbf{0.98} & -0.79 \\
                \midrule
           E886 \(\sigma^p\) (NuSea) & 89 & 1.02&+0.13&0.97 &-0.20 \\
           E886 \(\sigma^{d}/2\sigma^p\) (NuSea) & 15 & 1.17 &+0.46& 1.42&+1.15 \\
           E605 \(\sigma^p\) & 85 & 0.38&-4.04 &0.37 & -4.11\\
           E906 \(\sigma^{d}/2\sigma^p\) (SeaQuest) & 6 & 0.59&-0.71&0.67 &-0.57 \\
          \midrule
           CDF $Z$ differential & 28 & 1.02 &+0.07&1.00 &+0.00\\
           D0  $Z$ differential & 28 & 0.98 &-0.07& 1.00&+0.00\\
           D0  $W$ muon asymmetry & 9 &1.23 &+0.48&1.48 &+1.02\\
                \midrule
         ATLAS low-mass DY 7\,TeV & 6 &1.21 &+0.36&1.21 &+0.36 \\
         ATLAS \(W, Z\) 7 TeV (${\cal L}=35\,{\rm pb}^{-1}$) & 30 & 0.78&-0.85& 0.78&-0.85 \\
         ATLAS \(W, Z\) 7 TeV (${\cal L}=4.6\,{\rm fb}^{-1}$) central& 46 & 1.39&+1.87& 1.44&+2.11\\
         ATLAS \(W, Z\) 7 TeV (${\cal L}=4.6\,{\rm fb}^{-1}$) forward&15 & 0.91&-0.25& 0.92&-0.22 \\
         ATLAS low-mass DY 2D 8 TeV&60 & 0.87&-0.71& 0.86&-0.77 \\
        ATLAS $\sigma^{\rm tot}_{W,Z}$13 TeV & 3 &0.38 &-0.76&0.40&-0.73 \\
        ATLAS $W^+$+jet 8 TeV   &15&1.26&+0.71 &1.24 &+0.66 \\       
        ATLAS $W^-$ +jet 8 TeV   &15&1.02&+0.05 &0.98 &-0.05 \\       

          ATLAS $Z$ $p_T$ 8 TeV $(p_T , m_{ll})$& 44 &0.91 &-0.42&0.91 &-0.42 \\
          ATLAS $Z$ $p_T$ 8 TeV $(p_T , y_Z)$ & 48 &0.70 &-1.47&0.68 &-1.57 \\
                \midrule
CMS $W$ electron asymmetry 7 TeV & 11 &1.48&+1.13&1.50 &+1.17 \\
CMS $W$ muon asymmetry 7 TeV & 11 &1.22 &+0.52&1.28 &+0.66 \\
CMS $W$ rapidity 8 TeV& 22 &1.36 &+1.19& 1.37&+1.23 \\
 CMS  \(Z_{p_T}\) 8 TeV  & 28 &0.83&-0.64&0.82&-0.67\\
                \midrule
LHCb \(Z\rightarrow ee\)  7\,TeV & 9 &0.69&-0.66&0.69&-0.66 \\
LHCb \(W,Z\rightarrow\mu\) 7\,TeV & 29 &0.99&-0.04&0.94&-0.23 \\
LHCb \(Z\rightarrow ee\)  8\,TeV &17  &1.24&+0.70&1.24&+0.70 \\
LHCb \(W,Z\rightarrow\mu\) 8\,TeV &30&0.85&-0.58&0.74&-1.0\\
LHCb \(Z\rightarrow ee\)  13\,TeV & 15 &1.58&+1.59&1.60&+1.64 \\
LHCb \(Z\rightarrow\mu\) 13\,TeV & 16 &1.36&+1.02&1.37&+1.05 \\
                \midrule
                \textbf{Total DY (excl. HM)} & \textbf{670} & \textbf{xx} & \textbf{xx}& & \\
                \midrule
                ATLAS high-mass DY 7 TeV (${\cal L}=49\,{\rm fb}^{-1}$)& 13 &0.40 &-1.53& 0.40&-1.53 \\
                ATLAS high-mass DY 2D 8 TeV & 46 & 0.94&-0.29&0.94&-0.29 \\
                CMS high-mass DY 2D 7 TeV & 117 &0.92&-0.61&0.92&-0.61 \\
                CMS high-mass DY 8 TeV & 41 &1.30 &+1.36&1.29 &+1.31 \\
                CMS high-mass DY 13 TeV & 43 &1.06 &+0.28&1.07 &+0.32 \\
                \midrule
                \textbf{Total DY (HM only)} & \textbf{260} & \textbf{xx} & \textbf{xx}& & \\
                \midrule
%                \textbf{Total (excl. HL-LHC)} & \textbf{4715} & \textbf{xx} & \textbf{xx}& & \\
%                \midrule
                HL-LHC CC \(e\)& 16 & 0.79 &-0.60 & 1.00 & +0.0 \\ %% SM vs  Wcont   | Wcont vs SM
                HL-LHC CC \(\mu\)& 16 & 0.55 & -1.27 & 0.74 & -0.74\\
                HL-LHC NC \(e\)& 12 & 1.63 & +1.54 & 1.61 &+1.49 \\
                HL-LHC NC \(\mu\)& 12 & 0.81 &-0.46 & 0.79 &-0.51  \\
                \midrule
                \textbf{Total HL-LHC only} & \textbf{56} &\textbf{0.92} &-0.42 & \textbf{1.03} &+0.16 \\
                \midrule
                \textbf{Total} & \textbf{4771} & \textbf{0.97} & -1.41 & \textbf{0.96} &-1.89 \\
                \bottomrule
        \end{tabular}
        \caption{Values of the \(\chi^2\) per data point across all datasets
        used in this study. We tabulate values for the baseline PDF set as well
        as those obtained in the contaminated PDF fit. \label{tab:chi2w000008}}
\end{table}
