# Supplementary material for: Precision phenomenology of the PDF-BSM interplay
Source: arXiv:2503.02827 source file (2025-03-04)
Supplement: Supplementary file 3 [file appendix_sr.tex]

% App
%%%%%%%%%%%%%%%%%%%%%%%%%%%%%%%%%%%%%%%%%%
\section{Kinematics}

In this appendix we want to settle in the \textit{clearest} way the kinematics and the structure of the equations that we want to regress. For kinematic variables $x$, $y$, $z$, we want to write \textit{precisely} equations like

\begin{equation}
    F(x, y, z) = f_1 (x, y) \left(f_2 (z) \cdot x - 2 y^2 \cdot f_3(x, z) + f_4 (y) \right),
\end{equation}

where we understand clearly the 'structure' of the equation (what is or isn't factorised, the algebraic operations involved, etc) and the variables upon which every function $F$, $\{f_i \}_{i=1}^{4}$ depend on (what enters and does not enter in the functions, and the kinematics of \textit{which} particle in the process is the relevant one: is the lepton, the lepton pair, the intermediate boson?)

\subsection{The centre-of-mass hadronic frame}

Let us compute the Born process (leading-order)
\begin{equation}
    q_i(p_1) + \bar{q}_i(p_2) \, \to \, \gamma^* \to  l^-(p_3) + l^+(p_4),
\end{equation}
where $i$ is the flavour index. \\
Let us write explicitly the momenta in the partonic centre-of-mass energy, then we will move into the hadronic centre-of-mass energy
\begin{align*}
p_1 &= \frac{\sqrt{\hat{s}}}{2}(+1,0,0,+1)\\
p_2 &= \frac{\sqrt{\hat{s}}}{2}(+1,0,0,-1)\\
p_3 &= \frac{\sqrt{\hat{s}}}{2}(+1,+\sin\theta,0,+\cos\theta)\\
p_4 &= \frac{\sqrt{\hat{s}}}{2}(+1,-\sin\theta,0,-\cos\theta),
\end{align*}
where $\hat{s}$ is the partonic centre-of-mass energy squared and $\theta$ is the angle between the outgoing leptons and the incoming beams. Let us define the Mandelstam variables as
\begin{align*}
    \hat{s} & = (p_1+p_2)^2=(p_3+p_4)^2\\
    \hat{t} & = (p_1-p_3)^2 = (p_4 - p_2)^2 = -\frac{\hat{s}}{2}(1-\cos\theta)\\
    \hat{u} & = (p_1-p_4)^2 = (p_3 - p_2)^2 = -\frac{\hat{s}}{2}(1+\cos\theta)
\end{align*}
Computing the squared of the matrix element averaging/summing over the polarisation and colors, we get
\begin{equation}
    \overline{{\cal M}^2} = Q_i^2\alpha^2
    \frac{2^5\pi^2}{3}\frac{\hat{t}^2+\hat{u}^2}{\hat{s}^2} = Q_i^2\alpha^2
    \frac{2^4\pi^2}{3}(1+\cos^2\theta),
\end{equation}
where in the last passage we wrote $\hat{t}$ and $\hat{u}$ in terms of $\hat{s}$ and $\cos\theta$. The differential partonic cross section is given by
\begin{equation}
    d\hat{\sigma}^{(0)} = \frac{1}{2\hat{s}}\overline{{\cal M}^2} d\Pi_2,
\end{equation}
where $d\Pi_2$ is the two body massless phase space given by
\begin{equation}
 d\Pi_2=\frac{d^3p_3}{(2\pi)^32E_3}   \frac{d^3p_4}{(2\pi)^32E_4}(2\pi)^4\delta^{(4)}(p_1+p_2-p_3-p_4) = \frac{d\cos\theta}{16\pi}. 
\end{equation}
Putting everything together we get
\begin{equation}
\label{eq:pcs}
    \frac{d\hat{\sigma}^{(0)}}{d\cos\theta} = Q_i^2\alpha^2
    \frac{\pi}{6}\frac{1}{\hat{s}}(1+\cos^2\theta)
\end{equation}
and 
\begin{equation}
\label{eq:pcs_tot}
    \hat{\sigma}^{(0)} = Q_i^2\alpha^2
    \frac{4\pi}{9}\frac{1}{\hat{s}}
\end{equation}

Let us now go the the hadronic centre-of-mass frame (or laboratory frame as T. Han calls it in Ref.~\cite{Han:2005mu})
\begin{align*}
P_1 &= \frac{\sqrt{S}}{2}(+1,0,0,+1)\\
P_2 &= \frac{\sqrt{S}}{2}(+1,0,0,-1),
\end{align*}
where $p_1 = x_1P_1$ and $p_2 = x_2P_2$, so that
\begin{equation*}
    S = (P_1+P_2)^2 = \frac{\hat{s}}{x_1x_2} 
\end{equation*}
The factorisation theorem tells us that
\begin{align}
    \sigma(pp\to l^+l^-) &= \sum_{i}\int_{\tau^0}^1 dx_1\int_{\tau^0/x_1}^1 dx_2\, \left[q_i(x_1)\bar{q}(x_2)+q_i(x_2)\bar{q}_i(x_1)\right] \notag \\
    &\qquad\qquad \hat{\sigma}^{(0)}(q_i\bar{q}_i\to l^+l^-)
    \,\delta(x_1x_2-\tau^0),
\end{align}
where the $\delta$ functions comes because of the leading-order kinematics that constrains the product of $x_1$ and $x_2$ to be equal to $\tau^0=m_{ll}^2/S$, where $m_{ll}^2$ is the invariant mass of the outgoing lepton pair, which at the Born level is equal to the partonic centre-of-mass energy. 
Let us now define the rapidity in the hadronic centre-of-mass frame as
\begin{equation}
\label{eq:rap_def}
y = \frac{1}{2}\log\left(\frac{E_1+E_2+p^z_1+p^z_2}{E_1+E_2-(p^z_1+p^z_2)}\right)=\frac{1}{2}\log\left(\frac{x_1+x_2+x_1-x_2}{x_1+x_2-x_1+x_2}\right)=\frac{1}{2}\log(x_1/x_2).
\end{equation}
%%%%%%%%%%%%%%%%%%%%%
%Note that we can also express the rapidity of Eq. (\ref{eq:rap_def}) in terms of the kinematics of the final state and, in particular, in terms of the angle between the outgoing lepton and the incoming hadrons. To do this, we use conservation of momentum and write the rapidity as before

%\begin{equation*}
%y = \frac{1}{2}\log\left(\frac{E_3+E_4+p^z_3+p^z_4}{E_3+E_4-(p^z_3+p^z_4)}\right).
%\end{equation*}

%Since we are neglecting the masses of the particles, for each one we have $E_i^2 - |\vec{p}_i|^2 = m_i^2 = 0$, and therefore $E_i = |\vec{p}_i|$. We can write the $z$ component of each momentum of the leptons by projecting on the $Z$ axis (defined by the incoming hadrons) as ${p_z}_3 = |\vec{p}_3| \cos \theta = E_3 \cos \theta$. In this way, we have
%\begin{equation*}
%y = \frac{1}{2}\log\left(\frac{1 + \cos \theta}{1 - \cos \theta}\right).
%\end{equation*}

%However, for now, we come back to the rapidity in terms of the initial state kinematics.

%%%%%%%%%%%%%%%%%%%%% 

%%%%%%%%%%%%%%%%%%%%%%%%%%%%%
% MMA: completing this
Rapidity of the outgoing lepton-antilepton pair

\begin{equation}
    y = \frac{1}{2} \log(\frac{(E_3 + E_4) + (p_3^z + p_4^z)}{(E_3 + E_4) - (p_3^z + p_4^z)})
\end{equation}
In the parton c.o.m frame

\begin{equation}
    \begin{cases}
        E_3 = \gamma E (1 - \beta \cos \theta*) \\
        E_4 = \gamma E (1 + \beta \cos \theta*) \\
        p_3^z = \gamma E (\cos \theta* - \beta) \\
        p_4^z = \gamma E (\cos \theta* + \beta) \\
    \end{cases}
\end{equation}
We notice that

\begin{equation}
    \begin{cases}
        E_3 + E_4 = 2 \gamma E \\
        p_3^z + p_4^z = 2 \gamma E \cos \theta* \\
    \end{cases}
\end{equation}
We sustitute these results in the first Eq. and collect and simplify the common factor $2 \gamma E$ between the numerator and the denominator

\begin{equation}
    y = \frac{1}{2} \log(\frac{1 + \cos \theta*}{1 - \cos \theta*})
\end{equation}
Hence

\begin{equation}
    \frac{1 + \cos \theta*}{1 - \cos \theta*} = e^{2y}
\end{equation}
We want to express $\cos \theta*$ in terms of $y$

\begin{equation}
    \cos \theta* = \tanh(y)
\end{equation}
% completing this now
%%%%%%%%%%%%%%%%%%%%%%%%%%%%%

Using Eq. (\ref{eq:rap_def}) we can now make a change of variables $(x_1,x_2)\to(\tau,y)$,
\begin{equation}
   \tau = x_1x_2, y=\frac{1}{2}\log(x_1/x_2) \Longleftrightarrow x_1=\sqrt{\tau}e^{+y}, x_2=\sqrt{\tau}e^{-y},
\end{equation}
which gives $dx_1dx_2=d\tau d y$. The hadronic cross section becomes
\begin{align}
    \sigma(pp\to l^+l^-) &= \sum_{i}\int_{\tau^0}^1 d\tau \int_{1/2\log\tau}^{-1/2\log\tau} dy\, \left[q_i(\tau e^{+y})\bar{q}(\tau e^{-y})+q_i(\tau e^{-y})\bar{q}_i(\tau e^{+y})\right]\notag\\ 
    & \qquad\qquad \hat{\sigma}^{(0)}(q_i\bar{q}_i\to l^+l^-)
    \,\delta(\tau-\tau^0).
\end{align}
Using the $\delta$ function to set the leading-order constraint $\tau=\tau^0$ we have
\begin{equation}
  \sigma(pp\to l^+l^-) = \sum_{i} \int_{1/2\log\tau^0}^{-1/2\log\tau^0} dy\, \left[q_i(\tau^0 e^{+y})\bar{q}(\tau^0 e^{-y})+q_i(\tau^0 e^{-y})\bar{q}_i(\tau^0 e^{+y})\right] \hat{\sigma}^{(0)}(q_i\bar{q}_i\to l^+l^-)
\end{equation}
Substituting the expression we obtained in Eq.~\eqref{eq:pcs_tot} for the partonic cross section we obtain
\begin{align}
    \sigma(pp\to l^+l^-) &=  \frac{4\pi\alpha^2}{9} \frac{1}{m_{ll}^2}\notag\\
    &\sum_{i}Q_i^2 \int_{1/2\log\tau^0}^{-1/2\log\tau^0} dy\, \left[q_i(\tau^0 e^{+y})\bar{q}(\tau^0 e^{-y})+q_i(\tau^0 e^{-y})\bar{q}_i(\tau^0 e^{+y})\right],
\end{align}
where we substitute the $1/\hat{s}$ factor in the partonic cross section by $1/(\tau^0S) = 1/m_{ll}^2$. 

What happens if we want to be differential in the rapidity $y$ or in the angle $\theta$? First of all note that, given that $E_1+E_2=E_3+E_4=m_{ll}$ and

\subsection{The Collins-Soper frame}

The purpose of the Collins-Soper frame is to retain the factorised angular dependence on $(1+\cos^2\theta)$ even when one goes beyond the Born (leading-order) calculation. 

\subsection{Complete decomposition}

Below you find the complete differential distribution of lepton pair production via Z boson DY.

\begin{align}
\frac{d\sigma}{dp_T dy dm d\cos\theta d\phi} = \frac{3}{16\pi} \frac{d\sigma^{U+L}}{dp_T dy dm} \Bigg\{ & (1 + \cos^2\theta) + \frac{1}{2} A_0(1 - 3\cos^2\theta) + A_1 \sin 2\theta \cos \phi \nonumber \\
& + \frac{1}{2} A_2 \sin^2\theta \cos 2\phi + A_3 \sin\theta \cos\phi + A_4 \cos\theta \nonumber \\
& + A_5 \sin^2\theta \sin 2\phi + A_6 \sin 2\theta \sin \phi + A_7 \sin\theta \sin \phi \Bigg\}
\label{eq:full}
\end{align}

where, as explained above Eq. (\ref{eq:full}) in Ref.~\cite{ATLAS:2016rnf} we have

\begin{enumerate}
    \item $p_T$: transverse momentum of the Z boson,
    \item $y$: rapidity of the Z boson,
    \item $m$: invariant mass of the Z, boson\footnote{When working with MG events, the invariant mass distribution of the Z boson has to be found in terms of the invariant mass of the final state, with the lepton pair. This gives the distribution centered around $m_Z \approx 90$ GeV.},
    \item $\cos \theta$: cosine of the polar angle of the lepton,
    \item $\phi$: azimuthal angle of the lepton.
\end{enumerate}

Explicitly, the functional dependence is 

\begin{equation}
    \frac{d\sigma}{dp_T dy dm d\cos\theta d\phi} = \frac{d\sigma}{dp_T dy dm d\cos\theta d\phi}(p_T, y, m, \cos\theta, \phi),
\end{equation}

\begin{equation}
    \frac{d\sigma^{U+L}}{dp_T dy dm} = \frac{d\sigma^{U+L}}{dp_T dy dm} (p_T, y, m),
\end{equation}

\begin{equation}
    A_i = A_i (p_T, y, m),
\end{equation}

for $i = 0, \dots, 7$. Some considerations for Eq. (\ref{eq:full}):

\begin{enumerate}
    \item At LO, only $A_4$ is non zero.
    \item At NLO QCD ($\mathcal{O}(\alpha_s)$) $A_{0 - 3}$ become non-zero.
    \item The coefficients $A_{5, 6, 7}$ become non-zero, while remaining small, only at NNLO QCD ($\alpha_s^2$)
\end{enumerate}

Before we tackle the fully differential distribution in Eq. (\ref{eq:full}), we move through different levels of increasing complexity.

\subsection{Level 1: $e^+ \ e^- \to \gamma \to  \mu^+ \ \mu^-$}

In this case, the distribution (very well known, see for example Eq. (1.8) in P. and S.) is
\begin{equation}
    \frac{d\sigma}{d\Omega} = \frac{ \alpha^2}{4s}\left(1 + \cos^2\theta\right),
\end{equation}

where $d \Omega$ is a differential solid angle. The distribution has azimuthal symmetry (independent of $\phi$), so the only dependence is on $\cos \theta$. Explicitly, 

\begin{equation}
    \frac{d\sigma}{d\Omega} = \frac{d\sigma}{d\Omega} (\cos \theta),
\end{equation}

\begin{equation}
    \frac{ \alpha^2}{4s} = \text{constant},
\end{equation}

and the angular dependence is known. This concludes L1.

\subsection{Level 2: $p\ p \to \gamma \to \mu^+\mu^-$}

\begin{equation}
\frac{d\sigma}{dy dm d\cos\theta d\phi} = \frac{3}{16\pi} \frac{d\sigma^{U+L}}{dy dm} \left(1 + \cos^2\theta \right),
\label{eq:l2}
\end{equation}

where

\begin{enumerate}
    \item $y$: rapidity of the intermediate boson ($\gamma$), expressed as the average of the rapidities of the muon and antimuon.
    \item $m$: invariant mass of the intermediate boson ($\gamma$)\footnote{In terms of the lepton pair, as before.},
    \item $\cos \theta$: cosine of the polar angle of the lepton,
    \item $\phi$: azimuthal angle of the lepton.
\end{enumerate}

Explicitly, the functional dependence is 

\begin{equation}
    \frac{d\sigma}{dy dm d\cos\theta d\phi} = \frac{d\sigma}{dy dm d\cos\theta d\phi}(y, m, \cos\theta, \phi),
\label{eq:l2_angs}
\end{equation}

\begin{equation}
    \frac{d\sigma^{U+L}}{dy dm} = \frac{d\sigma^{U+L}}{dy dm} (y, m),
\end{equation}

Do you agree with this?

To compare the SR closed formula with the PDFs we have

\begin{equation}
    \frac{d^2\sigma}{dy_{ll}dm_{ll}} = \frac{8 \pi \alpha}{3 m_{ll}} \frac{1}{3 s} \left( 
\sum_{q} Q^2 (f_{q}(x_1) f_{\overline{q}} (x_2) + f_{\overline{q}}(x_1) f_{q}(x_2 ) \right),
\label{eq:l2_pdf}
\end{equation}

where $y_{ll}$ and $m_{ll}$ are, respectively, the rapidity and the invariant mass of the muon pair, $\alpha = e^2 /(4 \pi)$, $x_1 = \sqrt{\tau} e^y$, $x_2 = \sqrt{\tau} e^{-y}$, $\tau = m_{ll}^2 / s$.

\textbf{Question: how do we relate Eqs. (\ref{eq:l2_angs})  and (\ref{eq:l2_pdf})?}

\subsection{Level 3: $p \ p \to Z \to \mu^+ \mu^-$}

This case is a simplification of Eq. (\ref{eq:full}). It happens at LO, where only the annihilation diagram $q \overline{q} \to \ Z$ is present. In this case, only $A_4$ is non-zero and we have

\begin{equation}
\frac{d\sigma}{dy dm d\cos\theta d\phi} = \frac{3}{16\pi} \frac{d\sigma^{U+L}}{dy dm} \left\{  (1 + \cos^2\theta) + A_4 \cos\theta 
 \right\},
\label{eq:l3}
\end{equation}

where

\begin{enumerate}
    \item $y$: rapidity of the Z boson,
    \item $m$: invariant mass of the Z, boson\footnote{In terms of the lepton pair, as before.},
    \item $\cos \theta$: cosine of the polar angle of the lepton,
    \item $\phi$: azimuthal angle of the lepton.
\end{enumerate}

In this case, there is no $p_T$ of the Z boson. \manuel{let us discuss what happens with $m$ and $y$. We have a (peaked) invariant mass distribution but the rapidity of the $Z$ boson is infinite in this case...}

Explicitly, the functional dependence is 

\begin{equation}
    \frac{d\sigma}{dy dm d\cos\theta d\phi} = \frac{d\sigma}{dy dm d\cos\theta d\phi}(y, m, \cos\theta, \phi),
\end{equation}

\begin{equation}
    \frac{d\sigma^{U+L}}{dy dm} = \frac{d\sigma^{U+L}}{dy dm} (y, m),
\end{equation}

\begin{equation}
    A_4 = A_4 (y, m).
\end{equation}

Do you agree with this?

\section{Selection criteria and denoising}
\label{app:denoising}

PySR has three selection criteria options:
\begin{itemize}
    \item \texttt{accuracy}: selects the candidate model with the lowest loss.
    \item \texttt{best}: selects the candidate model with the highest score among expressions with a loss better than at least $1.5x$ the most accurate model. This is the default criterion.
    \item \texttt{score}: selects the candidate model with the highest score, defined as the negated derivative of the log-loss with respect to complexity.
\end{itemize}

Additionally, PySR has a denoising feature which can perform an optional preprocessing step that refines the input data using a Gaussian process with an adaptable kernel. This kernel is a composite of a Gaussian function for smoothing, a white noise component to address inherent noise, and a constant kernel to adjust the mean of the Gaussian process. The Gaussian process then provides denoised target values for each data point, which PySR then fits.

We can use the events of subsection \ref{subsec:l1} to evaluate the results that we obtain with the denoising feature. We show the equations that we obtain with PySR, according to the denoising options and the three  selection criteria, in tables \ref{tab:10bins}, \ref{tab:30bins}, and \ref{tab:100bins}, for 10, 30, and 100 bins, respectively. We see that, in general, the denoising Gaussian process leads to more convolved equations that miss the real distribution. Not using the denoising tends to lead to better performance. It is worth noting, however, that PySR can deal with noisy data in different ways. One alternative is to use a weighted loss that accounts for the uncertainty in each target value. 

\begin{table}[h]
\begin{center}
\begin{tabular}{@{}cl|l|l@{}}
\toprule
Denoise & \multicolumn{1}{c}{Accuracy} & \multicolumn{1}{c}{Best} & \multicolumn{1}{c}{Score} \\
\midrule
True & 
\begin{minipage}[t]{0.25\columnwidth}$0.0007090032 \cdot x_{0} + 9090.917$\end{minipage} & 
\begin{minipage}[t]{0.25\columnwidth}$9090.844 \cdot x_{0} \cdot (9.63109 \cdot 10^{-5} - 7.7957055 \cdot 10^{-5} \cdot x_{0}) \cdot (x_{0} - 0.22291435) + 9090.844$\end{minipage} & 
\begin{minipage}[t]{0.25\columnwidth}$0.20396256 \cdot x_{0} + 9090.812$\end{minipage} \\
\noalign{\smallskip} \hline \noalign{\smallskip}
False & 
\begin{minipage}[t]{0.25\columnwidth}$x_{0}^{2} \cdot (296.52358194355 \cdot x_{0}^{4} + 7046.0674) + 7613.42$\end{minipage} & 
\begin{minipage}[t]{0.25\columnwidth}$7250.1396 \cdot x_{0}^{2} + 7589.319$\end{minipage} & 
\begin{minipage}[t]{0.25\columnwidth}$7250.1396 \cdot x_{0}^{2} + 7589.319$\end{minipage} \\
\bottomrule
\end{tabular}
\caption{SR results for 10 bins.}
\label{tab:10bins}
\end{center}
\end{table}

\begin{table}[h]
\begin{center}
\begin{tabular}{@{}cc|c|c@{}}
\toprule
Denoise & Accuracy & Best & Score \\
\midrule
True & 
\begin{minipage}[t]{0.25\columnwidth}$-0.21235736(x_{0}-1.1249065)(2x_{0}-1.1303912)(2x_{0}+0.2443421) + 3225.8237$\end{minipage} & 
\begin{minipage}[t]{0.25\columnwidth}$0.024268737x_{0}^{2} + 3225.7983$\end{minipage} & 
\begin{minipage}[t]{0.25\columnwidth}$x_{0}^{2}(-0.86325264x_{0}^{2} + x_{0}) + 3225.7295$\end{minipage} \\
\noalign{\smallskip} \hline \noalign{\smallskip}
False & 
\begin{minipage}[t]{0.25\columnwidth}$x_{0}^{2}(123.43398x_{0}^{4}+2326.98053420264)+2538.3494$\end{minipage} & 
\begin{minipage}[t]{0.25\columnwidth}$2417.7627x_{0}^{2} + 2527.635$\end{minipage} & 
\begin{minipage}[t]{0.25\columnwidth}$2415.3643x_{0} + 2125.6453$\end{minipage} \\
\bottomrule
\end{tabular}
\caption{SR results for 30 bins.}
\label{tab:30bins}
\end{center}
\end{table}

\begin{table}[h]
\begin{center}
\begin{tabular}{@{}cc|c|c@{}}
\toprule
Denoise & Accuracy & Best & Score \\
\midrule
True & 
\begin{minipage}[t]{0.25\columnwidth}$x_{0}^{2}(-1.615747x_{0}^{2}+2x_{0}-0.081652954)+995.048$\end{minipage} & 
\begin{minipage}[t]{0.25\columnwidth}$x_{0}(-0.46552044x_{0}^{4}+x_{0}-0.24463812)+995.06415$\end{minipage} & 
\begin{minipage}[t]{0.25\columnwidth}$995.1925$\end{minipage} \\
\noalign{\smallskip} \hline \noalign{\smallskip}
False & 
\begin{minipage}[t]{0.25\columnwidth}$x_{0}(207.340216x_{0}+428.81232)+109.830989048+750.30175$\end{minipage} & 
\begin{minipage}[t]{0.25\columnwidth}$726.08685x_{0}^{2}+757.9762$\end{minipage} & 
\begin{minipage}[t]{0.25\columnwidth}$725.2477x_{0}+637.3749$\end{minipage} \\
\bottomrule
\end{tabular}
\caption{SR results for 100 bins.}
\label{tab:100bins}
\end{center}
\end{table}

The denoising option proved to be effective just to fit the level 1 distribution with a $(1 + \cos^2 \theta)^{-1}$ reweighting to find the overall constant, as shown in Tab. \ref{tab:const}. With denoising, any selection criterion gives the correct constant answer. On the other hand, if the denoising is not applied PySR finds equations that are more expressive than the real law of Nature.

\begin{table}[h]
\begin{center}
\begin{tabular}{@{}l|c|c|c@{}}
\toprule
Denoise & Accuracy & Best & Score \\
\midrule
True & 
$6833.678$ & 
$6833.678$ & 
$6833.678$ \\
\noalign{\smallskip} \hline \noalign{\smallskip}
False & 
\begin{minipage}[t]{0.25\columnwidth}
$x_{0}^{2}(661.2393x_{0} - 706.5968)(x_{0}^{2} + x_{0}) + 7593.010$
\end{minipage} & 
\begin{minipage}[t]{0.25\columnwidth}
$7614.049 - 194.01741x_{0}$
\end{minipage} & 
\begin{minipage}[t]{0.25\columnwidth}
$7614.0547 - 194.02724x_{0}$
\end{minipage} \\
\bottomrule
\end{tabular}
\caption{SR equations with denoising for the reweighted distribution.}
\label{tab:const}
\end{center}
\end{table}

The SR results are consistent even if we change the number of events of the dataset ($10^4$ or $10^5$, for example) and obtain different levels of statistical uncertainty.

It is reassuring that, even if we do not input our knowledge of the Natural law by reweighting the level 1 distribution, PySR is still clever enough to find the correct functional form in spite of the noise in the data.
%%%%%%%%%%%%%%%%%%%%%%%%%%%%%%%%%%%%%%%%%%%
