# Supplementary material for: Precision phenomenology of the PDF-BSM interplay
Source: arXiv:2503.02827 source file (2025-03-04)
Supplement: Supplementary file 4 [file app-bench.tex]

\section{Benchmarking with  SMEFiT}
\label{app:benchmark}

Here we  benchmark the performance of \simunet{} when operating
as a fixed-PDF EFT fitter, by means of a tuned comparison with
the {\sc\small SMEFiT} framework when identical theory and experimental inputs
are used in both cases.
\smefit currently provides two strategies to determine posterior
distributions in the EFT parameter space. The first, known as MCfit, is based on the Monte Carlo
replica method followed by parameter optimisation (as similarly used in \simunet{}).
The second is based on Nested Sampling (NS), a purely Bayesian approach for parameter inference.
At the linear EFT level, \smefit results based on MCfit and NS are identical~\cite{Ethier:2021bye}.
At the quadratic level~\cite{Giani:2023gfq},
however, the MCfit approach is affected by the potential pitfalls described in App.~\ref{app:quad},
which also prevent the use of \simunet{} for joint SMEFT-PDF fits in the presence
of quadratic EFT corrections.
We demonstrate now that, for a  linear EFT determination and a common choice of inputs, 
the results obtained using the two frameworks display excellent agreement.

Fig.~\ref{fig:simunet-vs-smefit-linear} displays this comparison between the
marginalised 95\% CL intervals of \simunet{}
and {\sc\small SMEFiT} (operating in the Nested Sampling mode) for a linear EFT fit that takes as input
in both cases the full dataset discussed in this work as well as the same SM and EFT
theory calculations (and hence also the same operator basis).
To ensure identical inputs, a parser has been written that automatically converts data and theory files
from the \simunet{} to the  {\sc\small SMEFiT} standard formats.
 The \simunet{} results displayed here coincide with those
 displayed in Fig.~\ref{fig:smeft_simu_bounds} in the fixed-PDF EFT analysis.
 Satisfactory agreement between the two fitting frameworks is obtained,
 and similar benchmarks have been successfully performed for other variants
 of the fixed-PDF EFT fits presented in this work.

%-----------------------------------------
\begin{figure}[t]
        \centering
        \includegraphics[width=\linewidth]{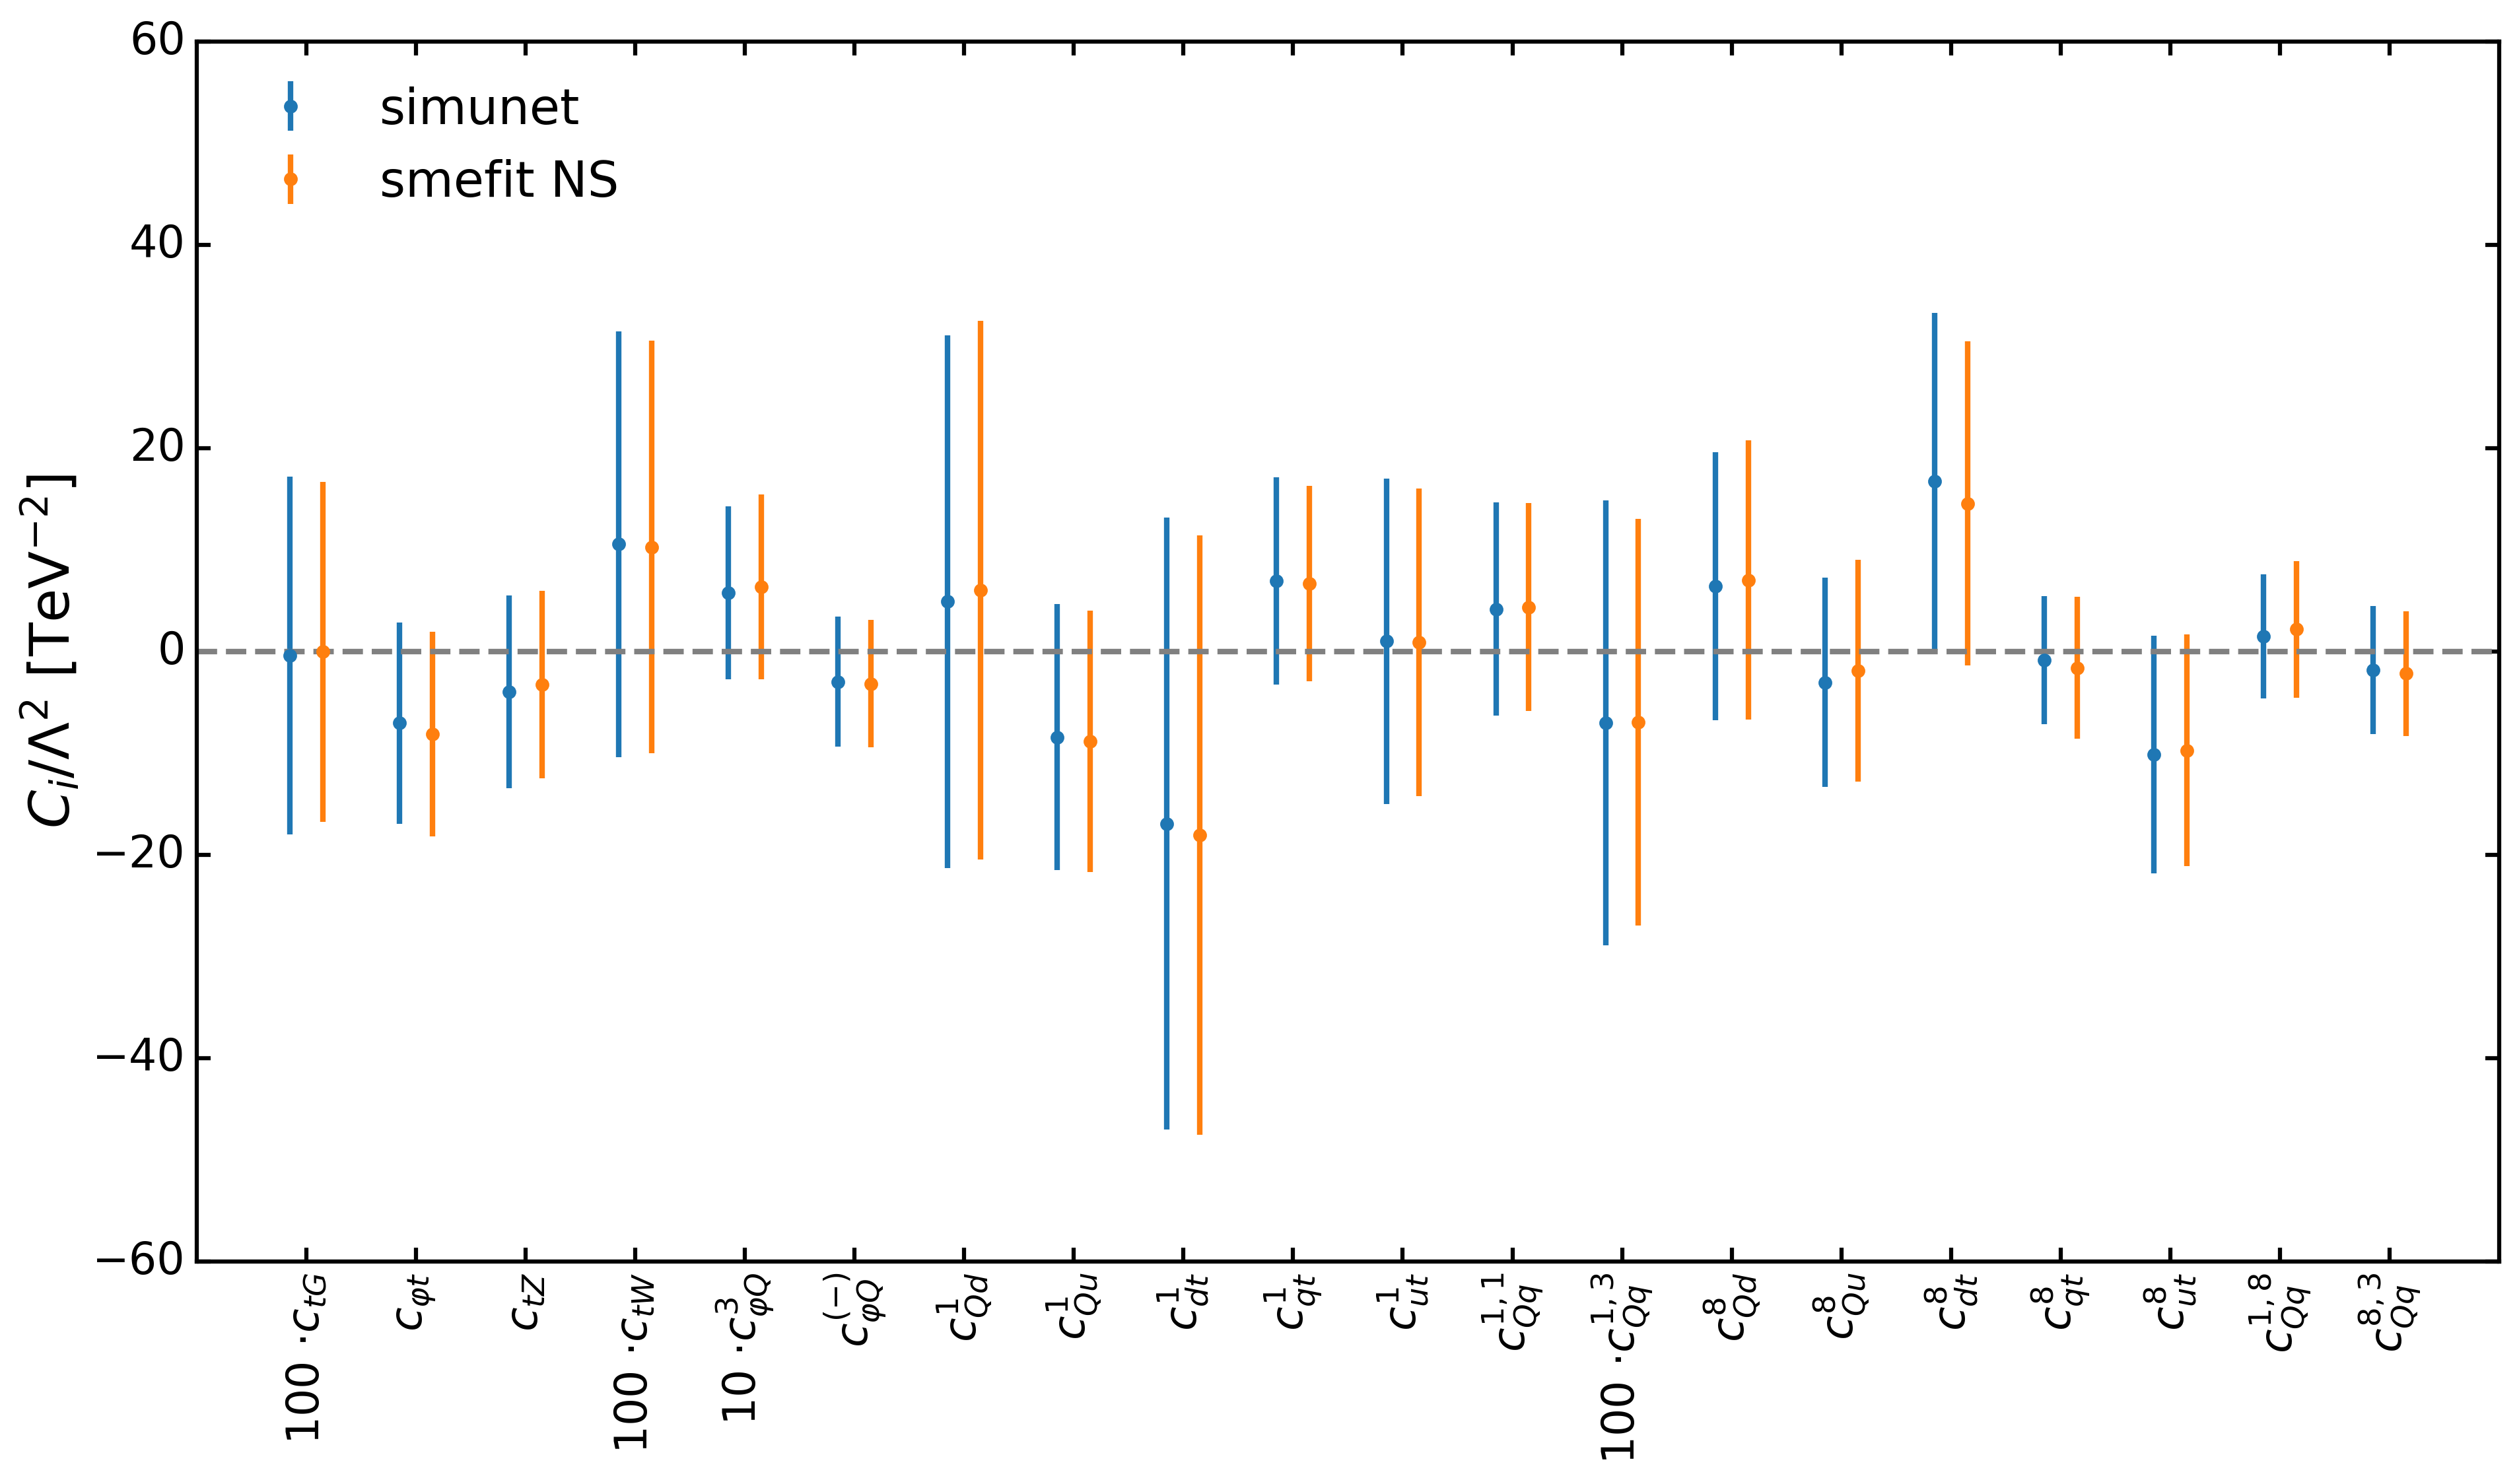}
	\caption{Comparison between the 95\% CL intervals
          obtained with \simunet{} in the fixed-PDF linear EFT case (full top quark dataset)
          with the corresponding results based on the {\sc\small SMEFiT}
          framework (with the Nested Sampling option).
          In both cases 
          the same experimental and theoretical inputs are adopted, see text for more details.
          These \simunet{} results coincide with those
          displayed in Fig.~\ref{fig:smeft_simu_bounds} in the fixed-PDF EFT analysis.
        }
	\label{fig:simunet-vs-smefit-linear}
\end{figure}
%-----------------------------------------

 This benchmark study ensures that the optimisation
 algorithm adopted by \simunet{} is suitable both for PDF determinations (since it is based
 on the NNPDF4.0 settings) as well as for the determination of the EFT coefficients.
 The optimisation settings that provide the best performance
 of the SM-PDF and fixed-PDF EFT analyses are then combined
 for the  simultaneous SMEFT-PDF extraction, where all weights of the \simunet{} network
 are allowed to be constrained by the data.

%\FloatBarrier
