# Supplementary material for: Precision phenomenology of the PDF-BSM interplay
Source: arXiv:2503.02827 source file (2025-03-04)
Supplement: Supplementary file 5 [file app-chi2sm.tex]

\section{Fit quality}
\label{app:fit_quality}

Here we summarise the $\chi^2$ (computed using the experimental
definition, Eq.~\ref{eq:chi2exp}) for the key PDF and EFT analyses presented in this work.
Tables~\ref{tab:chi2-baseline},~\ref{tab:chi2-top} and~\ref{tab:chi2-single-top} display
the values of the $\chi^2$ per data point for  representative PDF and EFT fits,
where for each dataset we also indicate the number of data points $n_{\rm dat}$.
Specifically, we consider: (i) three SM-PDF fits: \nnpdfnotop, \nnpdf, 
and Fit H in Table~\ref{tab:fit_list} (using our full top quark dataset);
(ii) two fixed-PDF EFT fits, one based on \nnpdfnotop as input,
and the other using Fit H as input; (iii) the outcome
of the simultaneous SMEFT-PDF determination.
We show sequentially the non-top datasets,
the $t\bar{t}$ inclusive and associated production datasets,
and the single-top inclusive and associated production datasets.
We also provide the total $\chi^2$ for separate groups of processes,
including the  full non-top and top datasets, and well as for their total sum.
    
In Tables~\ref{tab:chi2-top} and~\ref{tab:chi2-single-top},
entries in italics indicate datasets 
that do not enter the corresponding SM-PDF fit; for these datasets,
we evaluate the associated
$\chi^2$ values \textit{a posteriori} using the resulting PDFs.
For instance, all top data is removed from the \nnpdfnotop fit,
and for some top quark observables such as four-heavy-quark production,
PDF dependence is neglected.
Furthermore, we note that the $\chi^2$ values for the \nnpdfnotop fit
and for the fixed-PDF EFT fit based on \nnpdfnotop are identical
in Table~\ref{tab:chi2-baseline},
since the latter uses only top data as input.
For the same reason, the entries in the columns for the SM-PDF Fit H
and the fixed-PDF EFT fits based on Fit H are the same.
   
%%%%%%%%%%%%%%%%%%%%%%%%%%%%%%%%%%%%%%%
%%%%%%%%%%%%%%%%%%%%%%%%%%%%%%%%%%%%%%%%%%%%%%%%%%%%%%%%%%%%%%%%%%%%%%
\begin{table}[htbp]
  \begin{center}
  
%\scriptsize
\tiny
\begin{tabular}{ l | c| C{1.2cm} | C{1.2cm} | C{1.0cm} | C{1.2cm} | C{1.2cm} | C{1.2cm} }
 \toprule
 \multirow{3}{*}{Dataset}    & \multirow{3}{*}{$n_{\rm dat}$}   &  \multicolumn{6}{c}{$\chi^2/n_{\rm dat}$}  \\[1.5ex]
 &   & \multicolumn{3}{c|}{\bf SM-PDF fits} & \multicolumn{2}{c|}{\bf Fixed-PDF EFT fits}   & {\bf SMEFT-PDFs}    \\
  &   & NNPDF4.0 (no top)  & NNPDF4.0 & Fit H & NNPDF4.0 (no top) & Fit H & Joint fit   \\
 \midrule
 \midrule
 SLAC      & 67   & 0.768   & 0.758 & 0.753 & 0.768 & 0.753  & 0.761  \\
 BCDMS   & 581 &  	1.265  & 1.247 & 1.251 & 1.265  & 1.251  & 1.245   \\
 NMC       & 325 & 1.298   & 1.306 & 1.304  & 1.298  & 1.304  & 1.292    \\
 CHORUS  & 832 & 0.899    & 0.900 & 0.901  & 0.899  & 0.901  & 0.898     \\
  NuTeV     & 76  & 0.398 & 0.425  & 0.423 & 0.398  & 0.423  & 0.393    \\
 HERA  & 1208 & 1.204  & 1.203 & 1.204  & 1.204  & 1.204  & 1.200    \\
 \midrule
     {\bf Total DIS}  & {\bf 3089} &  {\bf 1.122 }  & {\bf 1.119 } & {\bf 1.119 } & {\bf 1.122 } & {\bf 1.119 } & {\bf 1.114 } \\
     \midrule
     \midrule
 E886    $\sigma^d_{\rm DY}/\sigma^p_{\rm DY}$ & 15  & 0.527    & 0.524  & 0.536  & 0.527 & 0.536   & 0.544   \\
 E886    $\sigma^p_{\rm DY}$                               & 89  & 1.566  & 1.559  & 1.615  & 1.566 & 1.615  & 1.602   \\
 E605   $\sigma^p_{\rm DY}$                                & 85  & 0.456   & 0.456  & 0.460 & 0.456  & 0.460  & 0.464    \\
 E906   $\sigma^d_{\rm DY}/\sigma^p_{\rm DY}$ &  6  &  0.827   &    0.885  & 0.886   & 0.827 & 0.886  &  0.955    \\
\midrule
{\bf Total fixed-target DY} & {\bf 195} & {\bf 0.981 } & {\bf 0.979 }   & {\bf 1.008 } & {\bf 0.981} & {\bf 1.008 } & {\bf 1.006 }  \\
 \midrule
 \midrule
 CDF    $d\sigma_Z/dy_Z$                                    & 28 &  1.234  & 1.280  &  1.275 & 1.234  & 1.275  & 1.188    \\
 D0     $d\sigma_Z/dy_Z$                                     & 28 &   0.637  & 0.644 &  0.640 & 0.637  & 0.640 & 0.632   \\
 D0    	$W\to \mu \nu$ asy.                       & 9  &   1.958 & 1.929 & 1.905  & 1.958  & 1.905 & 1.641     \\
 \midrule
 ATLAS low-mass DY 7 TeV               & 6 &  0.875  & 0.879 & 0.883  & 0.875  & 0.883 & 0.888    \\
 ATLAS high-mass DY 7 TeV               & 5 & 1.694 & 1.691 & 1.661 & 1.694  & 1.661 & 1.629  \\
 ATLAS $W, Z$ 7 TeV ($\mathcal{L} = 35$ pb${}^{-1}$) & 30   &  1.000 & 0.988 & 1.000 & 1.000 & 1.000  & 0.991    \\
 ATLAS  $W,Z$ 7 TeV ($\mathcal{L} = 4.6$ fb${}^{-1}$) & 61  & 1.689 & 1.686  & 1.685 & 1.685  & 1.685 & 1.599    \\
ATLAS low-mass DY 2D 8 TeV            & 60 & 1.203 &1.216 & 1.225 & 1.203  & 1.225 & 1.207   \\
ATLAS high-mass DY 2D 8 TeV           & 48 & 1.123  & 1.110 & 1.118 & 1.123  & 1.118 & 1.147   \\
ATLAS $\sigma_{W,Z}^{\rm tot}$ 13 TeV    & 3 & 0.727 & 0.778  & 0.706 & 0.727 & 0.706 & 0.471 \\
 \midrule
 CMS $W$ electron asymmetry 7 TeV             & 11 & 0.836 & 0.833 & 0.836 & 0.836 & 0.836 & 0.892   \\
CMS $W$ muon asymmetry 7 TeV              & 11 & 1.728 & 1.714 & 1.733 & 1.728  & 1.733 &  1.699  \\
CMS DY 2D 7 TeV                                        & 110 & 1.367 & 1.361 & 1.353 & 1.367 & 1.353 &  1.339 \\
CMS $W$ rapidity 8 TeV                              & 22 & 1.375 & 1.361 & 1.365 & 1.375  & 1.365 & 1.162  \\
 \midrule
 LHCb $Z \rightarrow ee$ 7 TeV                       & 9  &  1.630  & 1.648 & 1.636 & 1.630 & 1.636 & 1.669 \\
 LHCb $Z \rightarrow ee$ 8 TeV                        & 17  & 1.272   & 1.325 & 1.334 & 1.272 &  1.334 & 1.266 \\
 LHCb  $W,Z \rightarrow \mu$  7 TeV                 & 29  &   2.032 &  1.948 & 1.902 & 2.032 & 1.902 & 1.896   \\
 LHCb  $W,Z \rightarrow \mu$   8 TeV                & 30  & 1.494   & 1.426 & 1.417 & 1.494  & 1.417 & 1.386  \\
  LHCb  $Z \rightarrow ee$   13 TeV                & 15  & 1.701 & 1.726  & 1.717  & 1.701  & 1.717 & 1.640   \\
  LHCb  $Z \rightarrow \mu\mu$   13 TeV                & 16  & 0.970 & 0.993 & 0.978  & 0.970  & 0.978 & 0.928   \\
\midrule
{\bf Total inclusive gauge boson production} & {\bf 548} &  {\bf 1.344}  & {\bf 1.339}  & {\bf 1.335}  & {\bf 1.344}  & {\bf 1.335} & {\bf 1.297}    \\
 \midrule
 \midrule
ATLAS $W^{\pm}+$jet 8 TeV                      & 30 & 0.954 & 0.959 & 0.957  & 0.954  & 0.957 & 0.973 \\
ATLAS $Z$ $p_T$ 8 TeV ($p_T, m_{\ell\ell}$)      & 44 & 0.911 & 0.905 & 0.904 & 0.911 & 0.904 & 0.910 \\
ATLAS $Z$ $p_T$ 8 TeV ($p_T, y_Z$)                 & 48 & 0.909 & 0.898 & 0.896 & 0.909 & 0.896 & 0.924\\
ATLAS incl. jets 8 TeV, $R=0.6$                           & 171 & 0.682 & 0.687 & 0.687 & 0.682  & 0.687 & 0.667  \\
ATLAS dijets 7 TeV, $R=0.6$                               & 90 & 2.184  & 2.149  & 2.125  & 2.184 & 2.125 &. 2.177  \\
ATLAS isolated $\gamma$ prod. 13 TeV             & 53 & 0.811  & 0.763 & 0.753 & 0.811  & 0.753 & 0.813  \\
 \midrule
CMS $Z$ $p_T$ 8 TeV                                 & 28 & 1.447 & 1.401 & 1.407  & 1.447 & 1.407 & 1.473  \\
CMS incl. jets 8 TeV                                     & 185 & 1.140 & 1.183 & 1.200 & 1.140  & 1.200 & 1.118   \\
CMS dijets 7 TeV                                          & 54 & 1.788 & 1.810  & 1.809 & 1.788 & 1.809  & 1.800  \\
 \midrule
     {\bf Total jets, $Z$ $p_T$ and isolated photon}                      & {\bf 703} &  {\bf 1.154}  & {\bf 1.157} & {\bf 1.158}  & {\bf 1.154}  & {\bf 1.158}  & {\bf 1.148}  \\
      \midrule
 \midrule
     {\bf Total non-top data}                      & {\bf 4535} & {\bf 1.148}  &  {\bf 1.145} & {\bf 1.146} & {\bf 1.148} & {\bf 1.146} & {\bf 1.137} \\
 \bottomrule
\end{tabular}
\end{center}
  \caption{\small \label{tab:chi2-baseline} The values of the $\chi^2$ per data point (using the experimental
    definition of Eq.~\eqref{eq:chi2exp}) for key PDF and EFT analyses presented in this work.
    For each dataset, we indicate the number of data points $n_{\rm dat}$
    and the the $\chi^2$ values for {\it i)} three SM-PDF fits:
    \nnpdfnotop, \nnpdf,
    and Fit H in Table~\ref{tab:fit_list} (full top quark dataset);
    {\it ii)} two fixed-PDF EFT fits: one based on \nnpdfnotop as input,
    and the other using Fit H as input; and finally  {\it iii)} the outcome
    of the simultaneous SMEFT-PDF determination.
    Here we restrict ourselves to the non-top datasets considered in this
    analysis, the corresponding results for the top quark observables
    are provided in Tables~\ref{tab:chi2-top} and~\ref{tab:chi2-single-top}.
    We also provide the total $\chi^2$ for separate groups of processes as well
    as for the full non-top dataset.
    The $\chi^2$ values for the \nnpdfnotop fit
    and for the fixed-PDF EFT fit based on \nnpdfnotop are identical,
    since the latter uses only top data as input.
    For the same reason, the entries in the columns for the SM-PDF Fit H
    and the fixed-PDF EFT fits based on Fit H are the same.
}
\end{table}
%%%%%%%%%%%%%%%%%%%%%%%%%%%%%%%%%%%%%%%%%%%%%%%%%%%%%%%%%%%%%%%%%%%%%%%%%%
%%%%%%%%%%%%%%%%%%%%%%%%%%%%%%%%%%%%%%%%%%%%%%%%%%%%%%%%%%%%%%%%%%%%%%%%%%%%%%%%

%%%%%%%%%%%%%%%%%%%%%%%%%%%%%%%%%%%%%%%%
%%%%%%%%%%%%%%%%%%%%%%%%%%%%%%%%%%%%%%%%%%%%%%%%%%%%%%%%%%%%%%%%%%%%%%
\begin{table}[htbp]
  \begin{center}
  
%\scriptsize
  \tiny
\begin{tabular}{ l | c| C{1.2cm} | C{1.2cm} | C{0.8cm} | C{1.2cm} | C{1.0cm} | C{1.2cm} }
 \toprule
 \multirow{3}{*}{Dataset}    & \multirow{3}{*}{$n_{\rm dat}$}   &  \multicolumn{6}{c}{$\chi^2/n_{\rm dat}$}  \\[1.5ex]
 &   & \multicolumn{3}{c|}{\bf SM-PDF fits} & \multicolumn{2}{c|}{\bf Fixed-PDF EFT fits}   & {\bf SMEFT-PDFs}    \\
  &   & NNPDF4.0 (no top)  & NNPDF4.0 & Fit H & NNPDF4.0 (no top) & Fit H & Joint fit   \\
 \midrule
 \midrule
    ATLAS $\sigma(t\bar{t})$, dilepton, 7 TeV    & 1    &   \textit{4.100}  & 4.540 & 4.599 & 1.733 & 1.824 & 1.974     \\
    ATLAS $\sigma(t\bar{t})$, dilepton, 8 TeV & 1 & \textit{0.005} & 0.021 & 0.023 & 0.405 & 0.382 & 0.307 \\
    ATLAS $1/\sigma d\sigma/dm_{t\bar{t}}$, dilepton, 8 TeV & 5 & \textit{0.262} & \textit{0.284} & 0.291 & 0.305 & 0.309 & 0.310  \\
    ATLAS $\sigma(t\bar{t})$, $\ell+$jets, 8 TeV & 1 & \textit{0.218} & \textit{0.270} & 0.277 & 0.002 & 0.001  & 0.000  \\
    ATLAS $1/\sigma d\sigma/d|y_t|$, $\ell+$jets, 8 TeV & 4 & \textit{6.266} & 3.219 & 2.827 & 1.178 & 1.021 & 1.144 \\
    ATLAS $1/\sigma d\sigma/d|y_{t\bar{t}}|$, $\ell+$jets, 8 TeV & 4 & \textit{7.978} & 3.725 & 3.332 & 2.883 & 2.105 & 2.646  \\
    ATLAS $\sigma(t\bar{t})$, dilepton, 13 TeV           & 1    &  \textit{1.388}  & \textit{1.397}  & 1.374 & 0.004 & 0.004 & 0.002    \\
    ATLAS $\sigma(t\bar{t})$, hadronic, 13 TeV         & 1    & \textit{0.231}   &  \textit{0.231} & 0.230 & 0.082 & 0.082  & 0.092    \\
    ATLAS $1/\sigma d^2\sigma/d|y_{t\bar{t}}|dm_{t\bar{t}}$, hadronic, 13 TeV & 10 & \textit{2.276}  & \textit{2.007}  & 1.928 & 1.915 & 1.824 & 1.857  \\
    ATLAS $\sigma(t\bar{t})$, $\ell+$jets, 13 TeV & 1 & \textit{0.489} & 0.492 & 0.485 & 0.004 & 0.004 & 0.013 \\
    ATLAS $1/\sigma d\sigma/dm_{t\bar{t}}$, $\ell+$jets, 13 TeV & 8 & \textit{1.607} & \textit{1.788}  & 1.835 & 2.087 & 2.072 & 2.090  \\
    \midrule
    CMS $\sigma(t\bar{t})$, combined, 5 TeV & 1 & \textit{0.442}  & 0.542 & 0.555 & 0.211 & 0.236 & 0.239  \\
    CMS $\sigma(t\bar{t})$, combined, 7 TeV & 1 & \textit{0.795} & 1.032 & 1.065 & 0.004 & 0.010 & 0.027  \\
    CMS $\sigma(t\bar{t})$, combined, 8 TeV & 1 & \textit{0.170} & 0.247 & 0.258 & 0.174 & 0.156 & 0.103  \\
    CMS $1/\sigma d^2\sigma/d|y_{t\bar{t}}|dm_{t\bar{t}}$, dilepton, 8 TeV & 16 & \textit{1.094}  & \textit{0.994} & 0.963  & 0.519 & 0.580 & 0.514  \\
    CMS $1/\sigma d\sigma/d|y_{t\bar{t}}|$, $\ell+$jets, 8 TeV & 9 & \textit{2.127} &1.245 & 1.131 & 0.928 & 0.995 & 0.935  \\
    CMS $\sigma(t\bar{t})$, dilepton, 13 TeV & 1 & \textit{0.064}  & 0.063 & 0.066 & 0.680 & 0.680 & 0.600  \\
    CMS $1/\sigma d\sigma/dm_{t\bar{t}}$, dilepton, 13 TeV & 5 & \textit{2.760}  & 2.550 & 2.485 & 2.246 & 2.232 & 2.194  \\
    CMS $\sigma(t\bar{t})$, $\ell+$jets, 13 TeV & 1 & \textit{0.230} & \textit{0.227} & 0.234 & 2.153 & 2.155  & 1.907  \\
    CMS $1/\sigma d\sigma/dm_{t\bar{t}}$, $\ell+$jets, 13 TeV & 14 & \textit{1.829}  & \textit{1.481} & 1.393 & 0.962 & 0.911 & 0.912  \\
    \midrule
    ATLAS charge asymmetry, 8 TeV & 1 & \textit{0.679}  & \textit{0.678} & 0.675 & 0.567 & 0.587 & 0.571 \\
    ATLAS charge asymmetry, 13 TeV & 5 & \textit{1.012} & \textit{0.997} & 0.989 & 0.872 & 0.786 & 0.836 \\
    CMS charge asymmetry, 8 TeV & 3 & \textit{0.052} & \textit{0.052} & 0.053 & 0.072 & 0.069  & 0.071\\
    CMS charge asymmetry, 13 TeV & 3 & \textit{0.277} & \textit{0.283} & 0.286 & 0.443 & 0.510 & 0.451  \\
    ATLAS \& CMS combined charge asy., 8 TeV & 6 & \textit{0.603}  &\textit{0.602} & 0.602 & 0.646 & 0.659 & 0.651  \\
    \midrule
    ATLAS $W$-hel., 13 TeV & 2 & \textit{0.370} & \textit{0.370} & \textit{0.370} & 0.037 & 0.037 & 0.038   \\
    ATLAS \& CMS combined $W$-hel., 8 TeV & 2 & \textit{1.046} & \textit{1.046} & \textit{1.046} & 0.853 & 0.853 & 0.854  \\
       \midrule
   {\bf Total inclusive $t\bar{t}$}  & {\bf 108}  &  {\bf 1.700 } &  {\bf 1.328 } & {\bf 1.271 } & {\bf 1.032 } & {\bf 0.994} & {\bf 1.002 }  \\
     \midrule
     \midrule
    ATLAS $\sigma(t\bar{t}Z)$, 8 TeV & 1 & \textit{0.264}  &   \textit{0.232}  & 0.235 & 1.331 & 1.161 & 1.258 \\
    ATLAS $\sigma(t\bar{t}W)$, 8 TeV & 1 &  \textit{2.461} &  \textit{2.482} & 2.430 & 0.751 & 0.708 & 0.722   \\
    ATLAS $\sigma(t\bar{t}Z)$, 13 TeV & 1 &  \textit{0.702} &  \textit{0.747} & 0.742 & 0.001 & 0.000 & 0.000  \\
    ATLAS $1/\sigma d\sigma(t\bar{t}Z)/dp_T^Z$, 13 TeV & 5 &  \textit{1.961}  &  \textit{1.940} & 1.933 & 1.870 & 1.840 & 1.860  \\
    ATLAS $\sigma(t\bar{t}W)$, 13 TeV & 1 &  \textit{1.436} &  \textit{1.456} & 1.417 & 0.000 & 0.002 & 0.000 \\
    \midrule
    ATLAS $\sigma(t\bar{t}\gamma)$, 8 TeV & 1 & \textit{0.426} & \textit{0.426} & \textit{0.426} & 0.037 & 0.009 & 0.034  \\
    \midrule
    ATLAS $\sigma(t\bar{t}t\bar{t})$, multi-lepton, 13 TeV & 1 & \textit{3.655} & \textit{3.655} & \textit{3.655} & 4.289 & 3.784 & 4.145  \\
    ATLAS $\sigma(t\bar{t}t\bar{t})$, single lepton, 13 TeV & 1 & \textit{0.872} & \textit{0.872} & \textit{0.872} & 0.997 & 0.898 & 0.969  \\
    ATLAS $\sigma(t\bar{t}b\bar{b})$, $\ell+$jets, 13 TeV & 1 & \textit{2.062} & \textit{2.062} & \textit{2.062} & 1.093 & 1.316 & 1.152  \\
       \midrule
    CMS $\sigma(t\bar{t}Z)$, 8 TeV & 1 &  \textit{0.432}  &  \textit{0.470} & 0.466 & 0.005 & 0.020 & 0.010 \\
    CMS $\sigma(t\bar{t}W)$, 8 TeV & 1 &  \textit{2.281}  &  \textit{2.298} & 2.255 & 0.808 & 0.770 & 0.783  \\
    CMS $\sigma(t\bar{t}Z)$, 13 TeV & 1 &  \textit{1.185}  &  \textit{1.238} & 1.233 & 0.085 & 0.113 & 0.110 \\
    CMS $1/\sigma d\sigma(t\bar{t}Z)/dp_T^Z$, 13 TeV & 3 &  \textit{0.628}  &  \textit{0.598} & 0.590 & 0.936 & 0.756 & 0.898 \\
    CMS $\sigma(t\bar{t}W)$, 13 TeV & 1 &  \textit{0.667} &  \textit{0.682} & 0.652 & 0.297 & 0.329 & 0.307  \\
    \midrule
    CMS $\sigma(t\bar{t}\gamma)$, 8 TeV & 1 & \textit{0.508} & \textit{0.508} & \textit{0.508} & 0.022 & 0.045 & 0.024 \\
    \midrule
    CMS $\sigma(t\bar{t}t\bar{t})$, multi-lepton, 13 TeV & 1 & \textit{0.027} & \textit{0.027} & \textit{0.027} & 0.124 & 0.041 & 0.096  \\
    CMS $\sigma(t\bar{t}t\bar{t})$, single lepton, 13 TeV & 1 & \textit{0.231} & \textit{0.231} & \textit{0.231} & 0.262 & 0.238 & 0.255 \\
    CMS $\sigma(t\bar{t}b\bar{b})$, all-jet, 13 TeV & 1 & \textit{1.878} & \textit{1.878} & \textit{1.878} & 1.334 & 1.466 & 1.369  \\
    CMS $\sigma(t\bar{t}b\bar{b})$, dilepton, 13 TeV & 1 & \textit{0.962} & \textit{0.962} & \textit{0.962} & 0.312 & 0.447 & 0.347  \\
    CMS $\sigma(t\bar{t}b\bar{b})$, $\ell+$jets, 13 TeV & 1 & \textit{0.900} & \textit{0.900} & \textit{0.900} & 0.135 & 0.269 & 0.167  \\
    \midrule
   {\bf Total associated $t\bar{t}$}  & {\bf 26}  &  {\bf 1.255 } &  {\bf 1.255 } & {\bf 1.246 } & {\bf 0.925 } & {\bf 0.888 } & {\bf 0.913 } \\
%     \midrule
%     \midrule
%   {\bf Total top}  & {\bf 260}  &   &    \\
%     \midrule
%     \midrule
%     {\bf Grand total across all non-top \& top data}   &  {\bf 4022} & 1.1623  & 1.1627  \\
 \bottomrule
\end{tabular}
\end{center}
  \caption{\small \label{tab:chi2-top}
    Same as Table~\ref{tab:chi2-baseline} now
    for the  inclusive and associated $t\bar{t}$ production datasets.
     Values in italics indicate datasets 
    that do not enter the corresponding SM-PDF fit: for those processes,
    we evaluate a posteriori the physical observables and the associated
    $\chi^2$ values using the resulting PDFs from the fit.
    For instance, top data is removed from the \nnpdfnotop,
    and for some top quark observables like $t\bar{t}t\bar{t}$ their
    PDF dependence is neglected.
      The last row indicates the total values adding together the non-top
    and top data contributions to the $\chi^2$.
}
\end{table}
%%%%%%%%%%%%%%%%%%%%%%%%%%%%%%%%%%%%%%%%%%%%%%%%%%%%%%%%%%%%%%%%%%%%%%%%%%
%%%%%%%%%%%%%%%%%%%%%%%%%%%%%%%%%%%%%%%%%%%%%%%%%%%%%%%%%%%%%%%%%%%%%%%%%%%%%%%%

%%%%%%%%%%%%%%%%%%%%%%%%%%%%%%%%%%%%%%%
\begin{table}[htbp]
  \begin{center}
  
%\scriptsize
    \tiny
\begin{tabular}{ l | c| C{1.2cm} | C{1.2cm} | C{1.0cm} | C{1.2cm} | C{1.2cm} | C{1.5cm} }
 \toprule
 \multirow{3}{*}{Dataset}    & \multirow{3}{*}{$n_{\rm dat}$}   &  \multicolumn{6}{c}{$\chi^2/n_{\rm dat}$}  \\[1.5ex]
 &   & \multicolumn{3}{c|}{\bf SM-PDF fits} & \multicolumn{2}{c|}{\bf Fixed-PDF EFT fits}   & {\bf SMEFT-PDFs}    \\
  &   & NNPDF4.0 (no top)  & NNPDF4.0 & Fit H & NNPDF4.0 (no top) & Fit H & Joint fit   \\
 \midrule
 \midrule
     ATLAS $t$-channel $\sigma(t)$, 7 TeV & 1 & \textit{0.785} & \textit{0.756} & 0.757 & 0.179 & 0.135 & 0.155  \\
    ATLAS $t$-channel $\sigma(\bar{t})$, 7 TeV & 1 & \textit{0.304}  & \textit{0.296} & 0.282 & 0.003 & 0.005 & 0.004  \\
    ATLAS $t$-channel $1/\sigma d\sigma(tq)/dy_t$, 7 TeV & 3 & \textit{0.909} & 0.959 & 0.971 & 0.885 & 0.946 & 0.900  \\
     ATLAS $t$-channel $1/\sigma d\sigma(\bar{t}q)/dy_{\bar{t}}$, 7 TeV & 3 & \textit{0.061}  & 0.062 & 0.062 & 0.061 & 0.063 & 0.062  \\
     ATLAS $t$-channel $\sigma(t)$, 8 TeV & 1 & \textit{0.795}  & \textit{0.739} & 0.739 & 0.000 & 0.017 & 0.007 \\
     ATLAS $t$-channel $\sigma(\bar{t})$, 8 TeV & 1 & \textit{2.314} & \textit{2.277}  & 2.221 & 0.379 & 0.337 & 0.356  \\
    ATLAS $t$-channel $1/\sigma d\sigma(tq)/dy_t$, 8 TeV & 3 & \textit{0.288} & 0.246 & 0.241 & 0.290 & 0.245 & 0.283  \\
     ATLAS $t$-channel $1/\sigma d\sigma(\bar{t}q)/dy_{\bar{t}}$, 8 TeV & 3 & \textit{0.196} & 0.190 & 0.187 & 0.198 & 0.189 & 0.192  \\
     ATLAS $s$-channel $\sigma(t + \bar{t})$, 8 TeV & 1 & \textit{0.211} & \textit{0.203} & 0.216 & 0.000 & 0.000 & 0.000  \\
    ATLAS $t$-channel $\sigma(t)$, 13 TeV & 1 & \textit{0.738} & \textit{0.722} & 0.720 & 0.261 & 0.224 & 0.235  \\
    ATLAS $t$-channel $\sigma(\bar{t})$, 13 TeV & 1 & \textit{0.400} & \textit{0.393} & 0.384 & 0.057 & 0.050 & 0.051  \\
     ATLAS $s$-channel $\sigma(t + \bar{t})$, 13 TeV & 1 & \textit{0.700} & \textit{0.688} & 0.703 & 0.127 & 0.138 & 0.118  \\
    \midrule
    CMS $t$-channel $\sigma(t) + \sigma(\bar{t})$, 7 TeV & 1 & \textit{0.765}  & 0.729  & 0.719 & 0.010 & 0.001 & 0.004  \\
    CMS $t$-channel $\sigma(t)$, 8 TeV & 1 & \textit{0.010} & \textit{0.006} & 0.005 & 0.487 & 0.628 & 0.566  \\
    CMS $t$-channel $\sigma(\bar{t})$, 8 TeV & 1 & \textit{0.079} & \textit{0.084} & 0.092 & 0.886 & 0.934  & 0.911 \\
    CMS $s$-channel $\sigma(t + \bar{t})$, 8 TeV & 1 & \textit{1.108}  & \textit{1.112} & 1.105 & 1.348 & 1.338 & 1.350 \\
    CMS $t$-channel $\sigma(t)$, 13 TeV & 1 & \textit{0.904} & \textit{0.883} & 0.880 & 0.281 & 0.235 & 0.248  \\
    CMS $t$-channel $\sigma(\bar{t})$, 13 TeV & 1 & \textit{0.136} & \textit{0.132} & 0.125 & 0.010 & 0.014 & 0.013 \\
   CMS $t$-channel $1/\sigma d\sigma/d|y^{(t)}|$, 13 TeV & 4 & \textit{0.412} & \textit{0.387} & 0.383 & 0.405 & 0.378 & 0.396  \\
       \midrule
   {\bf Total single top}  & {\bf 30}  & {\bf 0.509 }  &  {\bf 0.498 } & {\bf 0.495 } & {\bf 0.332 } & {\bf 0.330 } & {\bf 0.331 }  \\
     \midrule
     \midrule
    ATLAS $\sigma(tW)$, dilepton, 8 TeV & 1 & \textit{0.510} & \textit{0.529} & 0.538 & 0.144  & 0.168 & 0.167 \\
    ATLAS $\sigma(tW)$, single-lepton, 8 TeV & 1 & \textit{0.695} & \textit{0.708} & 0.713 & 0.428 & 0.449 & 0.448  \\
    ATLAS $\sigma(tW)$, dilepton, 13 TeV & 1 & \textit{1.150} & \textit{1.149} & 1.148 & 0.840 & 0.847 & 0.849  \\
    ATLAS $\sigma_{\text{fid}}(tZj)$, dilepton, 13 TeV & 1 & \textit{0.115} & \textit{0.115} & \textit{0.115} & 0.871 & 0.611 & 0.795  \\
    \midrule
    CMS $\sigma(tW)$, dilepton, 8 TeV & 1 & \textit{0.359} & \textit{0.371} & 0.376 & 0.134 & 0.150 & 0.149 \\
    CMS $\sigma(tW)$, dilepton, 13 TeV & 1 & \textit{0.434} & \textit{0.437} & 0.438 & 1.612 & 1.573 & 1.563 \\
    CMS $\sigma_{\text{fid}}(tZj)$, dilepton, 13 TeV & 1 & \textit{1.041} & \textit{1.041} & \textit{1.041} & 0.279 & 0.427 & 0.316  \\
    CMS $d\sigma_{\text{fid}}(tZj)/dp_T^{t}$, dilepton, 13 TeV & 3 & \textit{0.362} & \textit{0.362} & \textit{0.362} & 0.130 & 0.156 & 0.134  \\
   CMS $\sigma(tW)$, single-lepton, 13 TeV & 1 & \textit{2.837} & \textit{2.833} & 2.832 & 1.817 & 1.839 & 1.846  \\
    \midrule
   {\bf Total associated single top}  & {\bf 11}  & {\bf 0.748 }  & {\bf 0.752 } &  {\bf 0.753 }  & {\bf 0.592 } & {\bf 0.594 } & {\bf 0.594 } \\
     \midrule
     \midrule
   {\bf Total top}  & {\bf 175}  & {\bf 1.370}   & {\bf 1.139} & {\bf 1.102} & {\bf 0.868} & {\bf 0.839} & {\bf 0.848}    \\
     \midrule
     \midrule
     {\bf Total dataset}   &  {\bf 4710} & {\bf 1.156}  & {\bf 1.145} & {\bf 1.144} & {\bf 1.138} & {\bf 1.135} & {\bf 1.126}  \\
 \bottomrule
\end{tabular}
\end{center}
  \caption{\small \label{tab:chi2-single-top}
     Same as Table~\ref{tab:chi2-top} now
    for the  inclusive and associated single-top production datasets.
    Values in italics indicate datasets 
    that do not enter the corresponding fits: for those processes,
    we evaluate a posteriori the physical observables and the associated
    $\chi^2$ values using the resulting PDFs from the fit.
    The last row indicates the total values adding together the non-top
    and top data contributions to the $\chi^2$,
    and the next-to-last row the total top quark contribution.
}
\end{table}
%%%%%%%%%%%%%%%%%%%%%%%%%%%%%%%%%%%%%%%%%%%%%%%%%%%%%%%%%%%%%%%%%%%%%%%%%%
%%%%%%%%%%%%%%%%%%%%%%%%%%%%%%%%%%%%%%%%%%%%%%%%%%%%%%%%%%%%%%%%%%%%%%%%%%%%%%%%

%%%%%%%%%%%%%%%%%%%%%%%%%%%%%%%%%%%%%%%

Several observations can be drawn
from the results presented in Tables~\ref{tab:chi2-baseline},~\ref{tab:chi2-top} and~\ref{tab:chi2-single-top}.
First of all, we note that the description of the non-top data is improved in the simultaneous
SMEFT-PDF analysis, with $\chi^2=1.137$ to be compared with the analogous SM-PDF analysis (Fit H)
which leads to $\chi^2=1.146$.
Given that we have $n_{\rm dat}=4535$ no-top data points, this
improvement corresponds to 40 units in the absolute $\chi^2$.
This improvement cannot be traced back to a specific measurements or group
of processes.
In turn, this improvement is also reflected for the full dataset,
whose $\chi^2$ is the lowest (1.126 for $n_{\rm dat}=4710$ points) in the SMEFT-PDF analysis.
This lower $\chi^2$ as compared to the SM-PDF baseline fits is not surprising,
taking into account the fact that (as discussed in Sect.~\ref{sec:res_smeft}) we now have more degrees
of freedom in the fit, and in particular the inclusion of linear EFT corrections
is instrumental in improving the $\chi^2$ to the top quark data as compared
to the SM-PDF fits.
We also find that the fit quality to the top datasets is similar in the joint SMEFT-PDF analysis
and in the fixed-PDF EFT fits with either \nnpdfnotop or Fit H as input
PDFs, with $\chi^2 = 0.848, 0.868, 0.839$ respectively in each case for
$n_{\rm dat}=175$.
The small differences between the three cases (less than five units
in absolute $\chi^2$) are consistent with the reported independence of the EFT interpretation
of top quark data with respect to the choice of input PDF in the calculation.

Finally, we note the only class of top quark production process for which the $\chi^2$ values
are markedly different in the SM-PDF fits is inclusive top quark pair production.
Indeed, the $\chi^2$ values for the complete top quark dataset are $1.370, 1.139$, and $1.102$ in the
SM-PDF fits without top data, with \nnpdf, and with the full top quark
dataset (Fit H) respectively; this improvement arises mostly from the $t\bar{t}$ group, whose $\chi^2$
values are $1.700, 1.328$, and $1.271$ for the same three fits respectively.
This observation is consistent with the findings of Sect.~\ref{sec:baseline_sm_fits}, that
the dominant PDF sensitivity in Fit H arises from inclusive $t\bar{t}$ production.
We also note that the $\chi^2$ for top quark data is similar between \nnpdf and Fit H, again
in agreement with the fact that the additional top quark measurements considered
here as compared to those in \nnpdf have a consistent pull on the PDFs, in particular
on the large-$x$ gluon.
