# Supplementary material for: Precision phenomenology of the PDF-BSM interplay
Source: arXiv:2503.02827 source file (2025-03-04)
Supplement: Supplementary file 6 [file app-quad.tex]

\section{Pitfalls of the Monte-Carlo replica method for quadratic EFT fits}
\label{app:quad}

This analysis was originally prepared with the intention of performing a fully simultaneous SMEFT-PDF
fit using NLO QCD theory, including \textit{quadratic}, $\mathcal{O}\lp \Lambda^{-4}\rp$, contributions from the SMEFT.
To this end, the capabilities of the \simunet{} framework were extended, as discussed in Sect.~\ref{sec:new_simunet}, and
all necessary SMEFT $K$-factors needed for the quadratic predictions were produced.
However, whilst benchmarking our code, we noticed significant disagreement between quadratic SMEFT-only fits
produced using the \simunet{} methodology and the \smefit Nested Sampling option;\footnote{This disagreement is not present at the linear level; in this case, \simunet{} using the fixed-PDF option and \smefit using either the Nested Sampling or MCfit options perfectly coincide. See App.~\ref{app:benchmark} for more details.} on the other hand, we note perfect agreement
between our \simunet{} quadratic SMEFT-only fits and the \smefit MCfit option.

This disagreement can be traced back to 
a deficiency in the Monte-Carlo sampling method used to propagate experimental error to the SMEFT coefficients, which
currently prevents us from applying the
the \simunet{} framework to joint SMEFT-PDF
fits with quadratic EFT calculations. 
In this Appendix, we describe our current understanding of these limitations within the context of a toy model, 
and give a more realistic example from this work; further work on the topic is deferred to a future publication..

\subsection{A toy model for quadratic EFT fits}
In the following subsection, we consider a toy scenario involving a single data point $d$ and only one
Wilson coefficient $c$ (we ignore all PDF-dependence).
We suppose that our observed experimental data point $d$ is a random variable drawn from a normal distribution
centred on the underlying quadratic theory prediction, and with experimental variance $\sigma^2$:
\begin{equation}
\label{eq:data_gaussian}
d \sim N(t(c), \sigma^2).
\end{equation}
We assume that the theory prediction is quadratic in the SMEFT Wilson coefficient $c$, taking the form:
\begin{equation}
t(c) = t^{\text{SM}} + c t^{\text{lin}} + c^2 t^{\text{quad}} \, ,
\end{equation}
where we set $\Lambda=1$ TeV for convenience. Recall that $t^{\text{quad}} > 0$, since it corresponds
to a squared amplitude.
Given the observed data $d$, we would like to construct interval estimates for the parameter
$c$ (usually \textit{confidence intervals} in a frequentist setting or \textit{credible intervals} in a Bayesian setting).
Here, we shall describe the analytical construction of two interval estimates: first, using the Bayesian method, and second, using the
Monte-Carlo replica method.

\paragraph{Bayesian method.}
In the Bayesian approach, $c$ is treated as a random variable with its own distribution. By Bayes'
theorem, we can write the probability distribution of $c$, given the observed data $d$, up to a proportionality constant (given by $1/\mathbb{P}(d)$, where $\mathbb{P}(d)$ is called the \textit{Bayes' evidence}) as:
\begin{equation}
\mathbb{P}(c | d) \propto \mathbb{P}(d | c) \mathbb{P}(c),
\end{equation}
\noindent
where $\mathbb{P}(c|d)$ is called the \textit{posterior distribution} of $c$, given the observed data $d$,
and  $\mathbb{P}(c)$ is called the \textit{prior distribution} of $c$ - this is our initial `best guess' of the distribution of $c$ before the observation
of the data takes place.
This distribution 
is often taken to be uniform in SMEFT fits; we shall assume this here.

Given a value of $c$, the distribution $\mathbb{P}(d|c)$ of the data $d$ is assumed to be Gaussian, as specified in Eq.~(\ref{eq:data_gaussian}). In particular, we can deduce that the posterior distribution of $c$ obeys the following proportionality relation:\footnote{Technically, truncated according to the end-points of the uniform prior.}
\begin{equation}
\label{eq:bayesian_posterior}
\mathbb{P}(c|d) \propto \exp\left( -\frac{1}{2\sigma^2} \left( d - t(c) \right)^2 \right).
\end{equation}
\noindent This posterior distribution can be used to place interval estimates on the parameter $c$. One way of doing this is to construct \textit{highest density intervals}. These are computed as follows.
For a $100\alpha$\% credible interval, we determine the constant $p(\alpha)$ satisfying:
\begin{equation}
\int\limits_{\{c : ~\mathbb{P}(c|d) > p(\alpha)\}} \mathbb{P}(c|d)\ dc = \alpha.
\end{equation}
\noindent An interval estimate for $c$ is then given by $\{c : \mathbb{P}(c|d) > p(\alpha)\}$. In order to obtain such intervals then, we must construct the posterior $\mathbb{P}(c|d)$; efficient sampling from the posterior
is guaranteed by methods such as Nested Sampling~\cite{Feroz:2013hea,Feroz:2007kg}.

\paragraph{The Monte-Carlo replica method.}
This method takes a different approach in order to produce a posterior distribution for the parameter $c$.
Given the observed central data value $d$, one samples repeatedly from the normal distribution $N(d, \sigma^2)$ to generate a collection of \textit{pseudodata replicas}, which we shall denote as $d^{(1)}, ..., d^{(N_{\text{rep}})}$, where $N_{\text{rep}}$ is the total number of replicas.
Given a pseudodata replica $d^{(i)}$, one obtains a corresponding best-fit value of the Wilson coefficient parameter $c^{(i)}$ by minimising the $\chi^2$ of the theory to the pseudodata:
\begin{equation}
c^{(i)} = \argmin_{c} \chi^2(c,d^{(i)}) = \argmin_{c} \left( \frac{(d^{(i)} - t(c))^2}{\sigma^2} \right).
\end{equation}
In this toy scenario, we can determine an analytical formula for $c^{(i)}$:
\begin{equation}
  c^{(i)} = \begin{cases} \displaystyle -\frac{t^{\text{lin}}}{2t^{\text{quad}}}, & \text{if $d^{(i)} \leq \lp t^{\text{SM}} - (t^{\text{lin}})^2/4t^{\text{quad}}\rp $ ;} \label{eq:app1} \\[2ex]
    \displaystyle \frac{-t^{\text{lin}} \pm \sqrt{(t^{\text{lin}})^2 - 4t^{\text{quad}}(t^{\text{SM}} - d^{(i)})}}{2t^{\text{quad}}}, & \text{if $d^{(i)} \geq \lp t^{\text{SM}} - (t^{\text{lin}})^2/4t^{\text{quad}}\rp $  \, .} \end{cases}
\end{equation}
The first case arises when the $\chi^2$ to the pseudodata $d^{(i)}$ has a single minimum, whilst the second case arises when the $\chi^2$  has two minima.
The two cases are split based on the value of
\be
\label{eq:crosssec_minimum}
t_{\text{min}} = t^{\text{SM}} - (t^{\text{lin}})^2/4t^{\text{quad}} \, ,
\ee
which is the minimum value of the quadratic theory prediction $t(c) = t^{\text{SM}} + c t^{\text{lin}} + c^2 t^{\text{quad}}$. Note that for data replicas such that $d^{(i)}\le t_{\text{min}}$, the best-fit value $c^{(i)}$
becomes independent of $d^{(i)}$ and depends only on the ratio between linear and quadratic
EFT cross-sections.

Now, given that $d^{(i)}$ is a random variable drawn from the normal distribution $N(d,\sigma^2)$, one can infer the corresponding distribution of the random variable $c^{(i)}$, which is a function of the pseudodata $d^{(i)}$.
For a real random variable $X$ with associated probability density $P_X(x)$, a function $f : \mathbb{R} \rightarrow \mathbb{R}$ of the random variable has the distribution:
\begin{equation}
P_{f(X)}(y) = \int\limits_{-\infty}^{\infty} dx\ P_X(x) \delta(y - f(x)).
\end{equation}
In our case, $c^{(i)}$ is a multi-valued function of $d^{(i)}$ given the two square roots, but the formula is easily generalised to this case.
Recalling that the pseudodata replicas are generated according
to a Gaussian distribution around the central measurement $d$ with variance $\sigma^2$,
we find that the probability density function for the Wilson coefficient replica
$c^{(i)}$ is given (up to a proportionality constant) by:
\begin{align}
P_{c^{(i)}}(c) &\propto \int\limits_{-\infty}^{t_{\text{min}}} dx\ \delta\left( c + \frac{t^{\text{lin}}}{2t^{\text{quad}}} \right) \exp\left( -\frac{1}{2\sigma^2} (x - d)^2 \right) \notag \\[1.5ex]
&\qquad + \int\limits_{t_{\text{min}}}^{\infty} dx\  \delta\left( c - \left(\frac{-t^{\text{lin}} + \sqrt{(t^{\text{lin}})^2 - 4t^{\text{quad}}(t^{\text{SM}} - x)}}{2t^{\text{quad}}}\right)\right)\exp\left( -\frac{1}{2\sigma^2} (x - d)^2 \right) \notag\\[1.5ex]
& \qquad + \int\limits_{t_{\text{min}}}^{\infty} dx\ \delta\left( c - \left(\frac{-t^{\text{lin}} - \sqrt{(t^{\text{lin}})^2 - 4t^{\text{quad}}(t^{\text{SM}} - x)}}{2t^{\text{quad}}}\right)\right) \exp\left( -\frac{1}{2\sigma^2} (x - d)^2 \right).
\end{align}
Simplifying the delta functions in the second and third integrals, we find:
\begin{equation}
\label{eq:mc_posterior}
P_{c^{(i)}}(c) \propto \delta\left( c + \frac{t^{\text{lin}}}{2t^{\text{quad}}} \right) \int\limits_{-\infty}^{t_{\text{min}}} dx\ \exp\left( -\frac{1}{2\sigma^2} (x - d)^2 \right) + \frac{2}{|2ct^{\text{quad}}  + t^{\text{lin}}|} \exp\left( -\frac{1}{2\sigma^2} (d - t(c))^2 \right) \, .
\end{equation}
This result is different from the posterior distribution obtained by the Bayesian method in Eq.~(\ref{eq:bayesian_posterior}). Notable features of the posterior distribution $P_{c^{(i)}}(c)$ are: (i) the distribution has a Dirac-delta peak at $c = -t^{\text{lin}}/2t^{\text{quad}}$; (ii) elsewhere, the distribution is given by the Bayesian posterior distribution rescaled by a prefactor dependent on $c$.
Therefore, the Monte Carlo
replica optimisation method will not in general reproduce the Bayesian posterior.

However, one can note that in an appropriate limit, the Bayesian posterior \textit{is} indeed recovered.
In particular, suppose that the quadratic EFT cross-section is subdominant
compared to the linear term, $t^{\text{lin}} \gg t^{\text{quad}}$; in this case, we have that
$t_{\text{min}} \rightarrow -\infty$ so that the first term in Eq.~\eqref{eq:mc_posterior} vanishes
and the prefactor of the second term can be approximated with $2ct^{\text{quad}} + t^{\text{lin}} \approx t^{\text{lin}}$. 
Thus, the Bayesian posterior from Eq.~(\ref{eq:bayesian_posterior}) is indeed recovered, and we 
see that the two methods are formally identical for a linear EFT analysis.
Further, it is possible to show analytically that for multiple SMEFT parameters and multiple correlated data points, 
if only linear theory is used the two distributions agree exactly.

%However, one can note that in appropriate limits, the Bayesian posterior \textit{is} indeed recovered. For example, in the case that  i.e. the case in which the quadratic terms are weaker compared to the linear terms, we find that Hence the first term in Eq.~(\ref{eq:mc_posterior}) vanishes, whilst the denominator of the prefactor in the second term approaches $2ct^{\text{quad}} + t^{\text{lin}} \approx t^{\text{lin}}$. Indeed, more generally, one can show that for multiple SMEFT parameters and multiple correlated data points, if only linear theory is used the two distributions agree exactly.\\
%\noindent Using the identity:
%\begin{equation}
%\int\limits_{t_{\text{\min}}}^{\infty} dx\ \exp\left( -\frac{1}{2\sigma^2} (x - d)^2 \right) = \sqrt{2\pi \sigma^2} - \int\limits_{-\infty}^{t_{\text{min}}} dx\ \exp\left( -\frac{1}{2\sigma^2} (x - d)^2 \right),
%\end{equation}
%\noindent we have:
%\begin{equation}
%P_{c^{(i)}}(c) \propto \left(\delta\left( c + \frac{t^{\text{lin}}}{2t^{\text{quad}}} \right) -\frac{2 }{2ct^{\text{quad}}  + t^{\text{lin}}} \right) \int\limits_{-\infty}^{t_{\text{min}}} dx\ \exp\left( -\frac{1}{2\sigma^2} (x - d)^2 \right) + \frac{2\sqrt{2\pi \sigma^2}}{2ct^{\text{quad}}  + t^{\text{lin}}}.
%\end{equation}

This calculation demonstrates that, for quadratic EFT fits, the Monte-Carlo replica method
will not in general reproduce the Bayesian posteriors that one would obtain from, say, a 
nested sampling approach; agreement will only occur provided quadratic EFT corrections 
are sufficiently subdominant in comparison with the linear ones.
For this reason, in this work we restrict the SMEFT-PDF fits based on \simunet{} (which rely
on the use of the Monte-Carlo replica method) to linear EFT calculations;
we defer the further investigation of the use of the Monte-Carlo replica method, and how
it might be modified for use in \simunet{}, to future works. 

%n the case where quadratic theory is used, the  cannot be expected to reliably reproduce the  distributions that one would obtain, say, from a nested sampling approach. It is for this reason that we choose to neglect quadratic contributions in our \simunet{} fits in this work; like \nnpdf and \smefit, \simunet{} assumes that the use of the Monte-Carlo method will produce a reliable posterior, but this is in fact not the case, and - as far as we are aware - has never been justified rigorously in the literature. In Section~\ref{subsec:mc_examples}, we give explicit examples of the failure of the Monte-Carlo method relative to the Bayesian method.

\subsection{Application to one-parameter fits}
\label{subsec:mc_examples}

As demonstrated above, the Monte-Carlo replica method will lead to
posterior distributions differing from their Bayesian counterparts whenever quadratic
EFT corrections dominate over linear ones.
Here, we show the numerical impact of these differences in a model case, namely
the one-parameter fit of the coefficient $c_{dt}^8$ to
the CMS 13 TeV $t\bar{t}$ invariant mass distribution measurement
based on the $\ell+$jets final-state~\cite{CMS:2021vhb}.
Fig.~\ref{fig:data-theory-CMS} compares the experimental data
from this measurement with the corresponding
SM theory calculations at NNLO using the NNPDF4.0 (no top) PDF
set as input.
We observe that the SM theory predictions overshoot the data, especially in the high $m_{t\bar{t}}$
regions, where energy-growing effects enhance the EFT corrections.
Given that the pseudodata replicas $d^{(i)}$ are fluctuated around the central value $d$,
the configuration where the SM overshoots the data
potentially enhances the contribution of the upper solution in Eq.~(\ref{eq:app1})
leading to the Dirac delta peak in the posterior Eq.~(\ref{eq:mc_posterior}).     

%-----------------------------------------
\begin{figure}[t]
        \centering
        \includegraphics[width=0.82\linewidth]{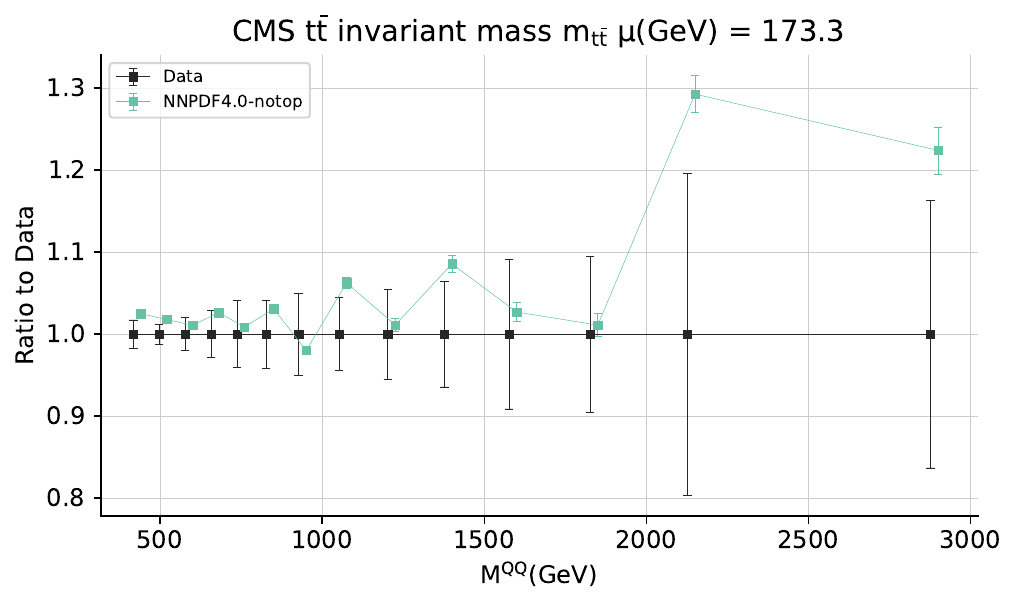}
        \caption{Comparison between the experimental data
          for the top-quark pair invariant mass $m_{t\bar{t}}$ distribution
          from the $\ell+$jets CMS measurement at 13 TeV~\cite{CMS:2021vhb}, with the corresponding
          SM theory calculations at NNLO using the NNPDF4.0 (no top) PDF
          set as input.
          For the latter, the error band indicates the PDF uncertainties, and
          for the former the diagonal entries of the experimental covariance matrix.
          Results are shown as ratios to the central value of the data.
          The SM theory predictions overshoot the data, especially in the high $m_{t\bar{t}}$
          regions, where energy-growing effects enhance the EFT corrections.
        }
    \label{fig:data-theory-CMS}
\end{figure}
%-----------------------------------------

For the case of the $c_{dt}^8$ coefficient, the quadratic EFT corrections dominate over the linear ones
and hence the net effect of a non-zero coefficient is typically an upwards shift
of the theory prediction.
Indeed, we have verified that for this coefficient
the biggest negative correction one can obtain is of order $\sim 2\%$.
For the last $m_{t\bar{t}}$ bin, the minimum of the  theory cross
section $t_{\rm min}$ in Eq.~(\ref{eq:crosssec_minimum}) is obtained for a value
$c_{dt}^8 \approx -0.2$, while for the second to last bin instead $t_{\rm min}$
is minimised by $c_{dt}^8 \approx -0.3$.
The combination of these two features (a dominant quadratic EFT term, and a SM prediction overshooting
the data) suggests that the Monte-Carlo replica method's
posterior will be enhanced for $c_{dt}^8 \in (-0.3,-0.2)$ as compared
to the Bayesian posterior.

%-----------------------------------------
\begin{figure}[h]
        \centering
        \includegraphics[width=0.49\linewidth]{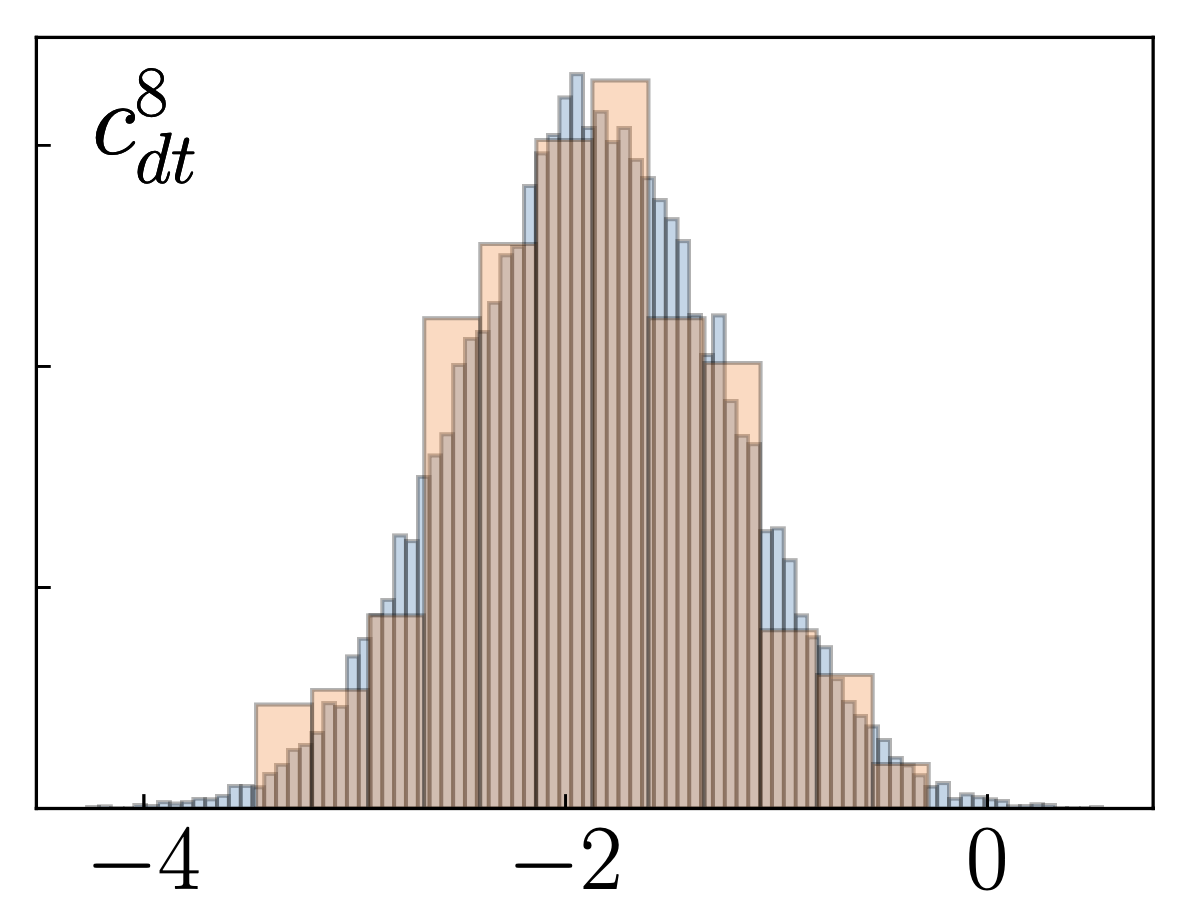}
        \includegraphics[width=0.49\linewidth]{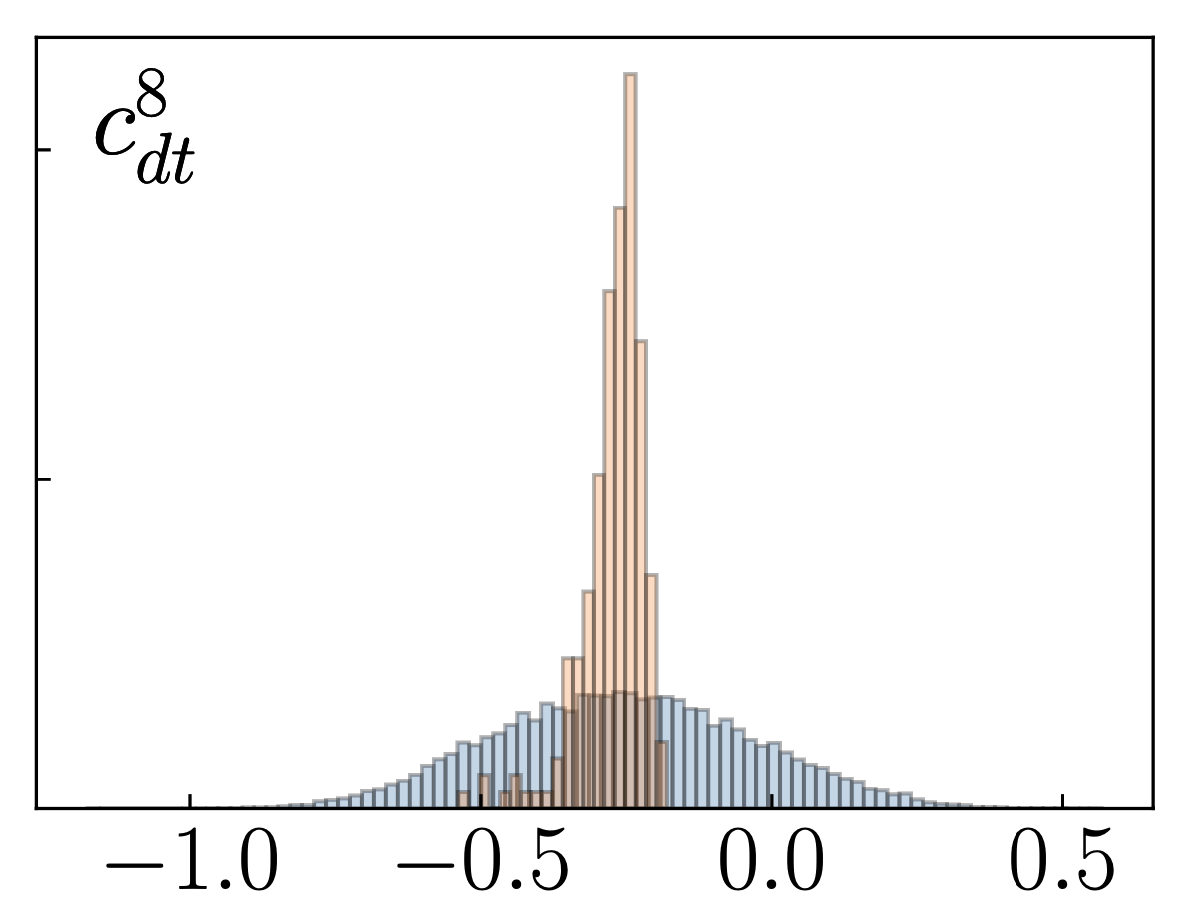}
        \caption{Posterior distributions for a one-parameter fit
          of the four-fermion coefficient $c_{dt}^8$ with the sole experimental
          input being the CMS $m_{t\bar{t}}$ distribution
          displayed in Fig.~\ref{fig:data-theory-CMS}.
          Results are obtained with \smefit and we compare the outcome of Nested Sampling (in blue) with
          that of MCfit (in red)
          for linear (left panel) and quadratic (right panel) EFT fits.
        }
    \label{fig:O8dt-fit}
\end{figure}
%-----------------------------------------

In Fig.~\ref{fig:O8dt-fit} we
compare the posterior distributions for a one-parameter fit
of the four-fermion coefficient $c_{dt}^8$ with the sole experimental
input being the CMS $m_{t\bar{t}}$ distribution
displayed in Fig.~\ref{fig:data-theory-CMS}.
Results are obtained with \smefit and we compare the outcome of Nested Sampling (in blue) with
that of MCfit (in red)
for linear and quadratic  EFT fits.
The agreement in the linear fit is lost for its quadratic counterpart,
with the main difference being a sharp peak in the region
$c_{dt}^8 \in (-0.3,-0.2)$ in which the contribution
from the delta function in Eq.~\ref{eq:mc_posterior} is most
marked.

The scenario displayed in Fig.~\ref{fig:O8dt-fit} is chosen to display the maximum effect,
based on a single coefficient with large quadratic EFT corrections, and a dataset
where the SM overshoots the data in the $m_{t\bar{t}}$ region where EFT effects
are the largest.
Within a global fit, these differences are \textit{partially} washed out
(indeed the Bayesian and MCfit posterior distributions mostly agree well for
the quadratic \smefit analysis, as shown in~\cite{Giani:2023gfq}, for the majority
of fitted coefficients).
Nevertheless, at least in its current implementation, Fig.~\ref{fig:O8dt-fit} highlights
that the Monte-Carlo replica method is affected by pitfalls that
prevent its straightforward application to global EFT interpretations of experimental
data which include quadratic corrections.
