# Supplementary material for: Precision phenomenology of the PDF-BSM interplay
Source: arXiv:2503.02827 source file (2025-03-04)
Supplement: Supplementary file 7 [file app-recommendations.tex]

\section{Recommendations to quantify SMEFT-PDF interplay}
\label{app:recommendations}

The strategy presented here, based on 
carrying out a simultaneous determination of the SMEFT-PDFs and the Wilson coefficients, makes possible a
quantitative assessment of the interplay between the PDF and SMEFT
sensitivity when interpreting a given set of LHC measurements. 
As discussed in Sect.~\ref{sec:summary}, the \simunet{} framework
will be made public only at a later stage.
In the meantime, researchers interested in quantifying this interplay in their
own analysis can use available open-source platforms like {\sc\small xFitter},
as done by the CMS collaboration
in their QCD and EFT analyses of double-differential inclusive jet cross sections
at 13 TeV~\cite{CMS:2021yzl}.
In several cases, however, a joint  analysis may not be necessary,
and one can estimate the possible role of the SMEFT-PDF interplay by means
of a simplified approach.
The discussion is presented here for the case of top quark measurements,
but it can be straightforwardly extended to any other class of measurements.

\begin{itemize}
\item The most conservative strategy is to introduce a hard boundary between those processes
  used for PDF fits and those entering SMEFT interpretations.
  For instance, for a SMEFT analysis of LHC top quark measurements one can use
  PDF fits without top data, such as the \nnpdfnotop variant.
  We recall that with the NNPDF open-source code~\cite{NNPDF:2021uiq} one can produce fit variants
  with arbitrary input datasets.

\item A somewhat less  conservative assumption would be to introduce a hard boundary,
  not at the process level, but rather at the kinematic level.
  In the case of inclusive top quark pair production data, one can introduce a threshold on the
  top quark pair invariant mass $m_{t\bar{t}}$ such that data points below the threshold
  are used for the PDF fit and above it for the EFT interpretation, thus
  benefiting from the increased sensitivity to BSM effects in the high-energy tails
  of the LHC distributions.
  Again, using public PDF fitting codes one can produce fit variants
  with tailored kinematical cuts to separate the ``PDF'' region from the ``EFT'' region.
  One drawback of this approach is that there is never a clear-cut separation
  between these regions; depending on the EFT operators considered,
  the high-energy region may not be the dominant one.

\item As demonstrated in this work, many measurements of relevance for EFT
  interpretations have limited sensitivity to PDFs and vice-versa.
  In such cases, the SMEFT-PDF interplay can be safely neglected.
  One can determine under which settings this condition is satisfied by
  adding the dataset under consideration either to a global PDF fit
  (using for example the NNPDF fitting code~\cite{NNPDF:2021uiq}) or to a global SMEFT
  fit (using the \smefit or \fitm frameworks).
  If the results of either the PDF or EFT fits are unchanged, one can safely neglect
  the SMEFT-PDF interplay in this case.

\item If instead the above analysis shows that a given dataset provides non-trivial information 
  on both the PDFs and on the EFT Wilson coefficients, the only options for a consistent
  theoretical interpretation are either introducing a hard boundary in the analysis (either
  at the process level or at the kinematic level) or to carry out
  the joint SMEFT-PDF interpretation of the full dataset using 
  \simunet{} or other available tools.

\end{itemize}

Furthermore, it should be emphasised that, as opposed to the PDF case,
the sensitivity to EFT coefficients of
a given measurement depends in general on the choice of EFT operator considered.
Hence, the above considerations assume a specific choice of operators and could be
different if this choice is varied.
