# Supplementary material for: Precision phenomenology of the PDF-BSM interplay
Source: arXiv:2503.02827 source file (2025-03-04)
Supplement: Supplementary file 8 [file app-theory.tex]

\section{EFT operator basis}
\label{sec:operators}

Table~\ref{tab:ops} lists the dimension-six
SMEFT operators relevant for this analysis, together with the corresponding
degrees of freedom (DoF) entering the fit.
In terms of the flavour assumptions, we follow the LHC top quark working group
recommendations~\cite{Aguilar-Saavedra:2018ksv},
which were also adopted in~\cite{Ethier:2021bye,Ellis:2020unq}.
The flavour symmetry group is
given by U(3)$_l \times$ U(3)$_e \times$ U(3)$_d \times$ U(2)$_u \times$ U(2)$_q$, i.e. one singles out operators that contain
top quarks (right-handed $t$ and SU(2) doublet $Q$).
This means that we work in a 5-flavour scheme, where the only massive fermion in the theory is the top quark.
The upper part in Table~\ref{tab:ops} defines the relevant two-fermion 
operators modifying the interactions of the third-generation
quarks.
We also indicate the notation used for the associated Wilson coefficients; those
in brackets are not degrees of freedom entering the fit,
and instead the two additional DoF defined in the middle table are used.
The bottom table defines the four-fermion DoF entering the fit,
expressed in terms of the corresponding four-fermion Wilson coefficients
associated to dimension-six SMEFT operators in the Warsaw basis.

EFT cross-sections at the linear and quadratic order in the EFT expansion
are computed for the datasets considered in this analysis
and for the DoF defined in Table~\ref{tab:ops}, both
at LO and NLO in perturbative QCD.
Furthermore we use the $m_W$-scheme,  meaning that the four EW inputs are
$\{m_W, G_F, m_h, m_Z\}$.
In particular, the electric charge $e$ becomes a dependent parameter and is shifted by 
the effects of higher-dimensional operators.

%%%%%%%%%%%%%%%%%%%%%%%%%%%%%%%%%%%%%%%%%%%%%%%%%%%%%%%%%%
\begin{table}[htbp]
  \begin{center}
    
    {\small
    \begin{tabular}{lll}
      \toprule
      Operator $\qquad$ & Coefficient & Definition \\
                \midrule
%%%%%%%%%%%%%%%%%%%%%%%%%%%%%%%%%%%%%%%%%%%%%%%%%%%%%%%%%%%%%%%%%%%%%%%%%%%
    $\Op{\varphi Q}^{(1)}$ & --~~($c_{\varphi Q}^{(1)}$) & $i\big(\varphi^\dagger\lra{D}_\mu\,\varphi\big)
 \big(\bar{Q}\,\gamma^\mu\,Q\big)$ \\\hline
%%%%%%%%%%%%%%%%%%%%%%%%%%%%%%%%%%%%%%%%%%%%%%%%%%%%%%%%%%%%%%%%%%%%%%%%%%%
    $\Op{\varphi Q}^{(3)}$ & $c_{\varphi Q}^{(3)}$  & $i\big(\varphi^\dagger\lra{D}_\mu\,\tau_{\sss I}\varphi\big)
 \big(\bar{Q}\,\gamma^\mu\,\tau^{\sss I}Q\big)$ \\ \hline
 %%%%%%%%%%%%%%%%%%%%%%%%%%%%%%%%%%%%%%%%%%%%%%%%%%%%%%%%%%%%%%%%%%%%%%%%%%%
    $\Op{\varphi t}$ & $c_{\varphi t}$& $i\big(\varphi^\dagger\,\lra{D}_\mu\,\,\varphi\big)
 \big(\bar{t}\,\gamma^\mu\,t\big)$ \\ \hline
%%%%%%%%%%%%%%%%%%%%%%%%%%%%%%%%%%%%%%%%%%%%%%%%%%%%%%%%%%%%%%%%%%%%%%%%%%%
      $\Op{tW}$ & $c_{tW}$ & $i\big(\bar{Q}\tau^{\mu\nu}\,\tau_{\sss I}\,t\big)\,
 \tilde{\varphi}\,W^I_{\mu\nu}
 + \text{h.c.}$ \\  \hline
%%%%%%%%%%%%%%%%%%%%%%%%%%%%%%%%%%%%%%%%%%%%%%%%%%%%%%%%%%%%%%%%%%%%%%%%%%%
 $\Op{tB}$ & --~~($c_{tB}$) &
 $i\big(\bar{Q}\tau^{\mu\nu}\,t\big)
 \,\tilde{\varphi}\,B_{\mu\nu}
 + \text{h.c.}$ \\\hline
%%%%%%%%%%%%%%%%%%%%%%%%%%%%%%%%%%%%%%%%%%%%%%%%%%%%%%%%%%%%%%%%%%%%%%%%%%%
    $\Op{t G}$ & $c_{tG}$ & $i\,\big(\bar{Q}\tau^{\mu\nu}\,T_{\sss A}\,t\big)\,
 \tilde{\varphi}\,G^A_{\mu\nu}
 + \text{h.c.}$ \\
 \bottomrule\\
 \toprule
      DoF $\qquad$  & Definition \\
                \midrule
$c_{\varphi Q}^{(-)}$ &  $c_{\varphi Q}^{(1)} - c_{\varphi Q}^{(3)}$ \\
\midrule
$c_{tZ}$ &   $-\sin\theta_W c_{tB} + \cos\theta_W c_{tW} $\\
  \bottomrule\\
 \toprule
          DoF $\qquad$ &  Definition (Warsaw basis) \\
          \midrule
      $c_{QQ}^1$    &   $2\ccc{1}{qq}{3333}-\frac{2}{3}\ccc{3}{qq}{3333}$ \\ \hline
%%%%%%%%%%%%%%%%%%%%%%%%%%%%%%%%%%5%%%%%%%%%%%%%%%%%%%%%%%%%%%%%%%%%%%%%%%%%%%%%%%%%%%%%%%%%%%%%%%%%%%%%%
    $c_{QQ}^8$       &         $8\ccc{3}{qq}{3333}$\\  \hline
          %%%%%%%%%%%%%%%%%%%%%%%%%%%%%%%%%%5%%%%%%%%%%%%%%%%%%%%%%%%%%%%%%%%%%%%%%%%%%%%%%%%%%%%%%%%%%%%%%%%%%%%%%
 $c_{Qt}^1$         &         $\ccc{1}{qu}{3333}$\\   \hline
          %%%%%%%%%%%%%%%%%%%%%%%%%%%%%%%%%%5%%%%%%%%%%%%%%%%%%%%%%%%%%%%%%%%%%%%%%%%%%%%%%%%%%%%%%%%%%%%%%%%%%%%%%
 $c_{Qt}^8$         &         $\ccc{8}{qu}{3333}$\\   \hline
          %%%%%%%%%%%%%%%%%%%%%%%%%%%%%%%%%%5%%%%%%%%%%%%%%%%%%%%%%%%%%%%%%%%%%%%%%%%%%%%%%%%%%%%%%%%%%%%%%%%%%%%%%
  $c_{tt}^1$         &     $\ccc{}{uu}{3333}$  \\    \hline
  %%%%%%%%%%%%%%%%%%%%%%%%%%%%%%%%%%5%%%%%%%%%%%%%%%%%%%%%%%%%%%%%%%%%%%%%%%%%%%%%%%%%%%%%%%%%%%%%%%%%%%%%%
 $c_{Qq}^{1,8}$       &      $\ccc{1}{qq}{i33i}+3\ccc{3}{qq}{i33i}$     \\   \hline
        %%%%%%%%%%%%%%%%%%%%%%%%%%%%%%%%%%5%%%%%%%%%%%%%%%%%%%%%%%%%%%%%%%%%%%%%%%%%%%%%%%%%%%%%%%%%%%%%%%%%%%%%%
  $c_{Qq}^{1,1}$         &   $\ccc{1}{qq}{ii33}+\frac{1}{6}\ccc{1}{qq}{i33i}+\frac{1}{2}\ccc{3}{qq}{i33i} $   \\    \hline
        %%%%%%%%%%%%%%%%%%%%%%%%%%%%%%%%%%5%%%%%%%%%%%%%%%%%%%%%%%%%%%%%%%%%%%%%%%%%%%%%%%%%%%%%%%%%%%%%%%%%%%%%%
   $c_{Qq}^{3,8}$         &   $\ccc{1}{qq}{i33i}-\ccc{3}{qq}{i33i} $   \\   \hline
        %%%%%%%%%%%%%%%%%%%%%%%%%%%%%%%%%%5%%%%%%%%%%%%%%%%%%%%%%%%%%%%%%%%%%%%%%%%%%%%%%%%%%%%%%%%%%%%%%%%%%%%%%
  $c_{Qq}^{3,1}$          &     $\ccc{3}{qq}{ii33}+\frac{1}{6}(\ccc{1}{qq}{i33i}-\ccc{3}{qq}{i33i}) $   \\     \hline
        %%%%%%%%%%%%%%%%%%%%%%%%%%%%%%%%%%5%%%%%%%%%%%%%%%%%%%%%%%%%%%%%%%%%%%%%%%%%%%%%%%%%%%%%%%%%%%%%%%%%%%%%%
   $c_{tq}^{8}$         &  $ \ccc{8}{qu}{ii33}   $ \\    \hline
        %%%%%%%%%%%%%%%%%%%%%%%%%%%%%%%%%%5%%%%%%%%%%%%%%%%%%%%%%%%%%%%%%%%%%%%%%%%%%%%%%%%%%%%%%%%%%%%%%%%%%%%%%
   $c_{tq}^{1}$       &   $  \ccc{1}{qu}{ii33} $\\    \hline
        %%%%%%%%%%%%%%%%%%%%%%%%%%%%%%%%%%5%%%%%%%%%%%%%%%%%%%%%%%%%%%%%%%%%%%%%%%%%%%%%%%%%%%%%%%%%%%%%%%%%%%%%%
   $c_{tu}^{8}$      &   $2\ccc{}{uu}{i33i}$  \\     \hline
        %%%%%%%%%%%%%%%%%%%%%%%%%%%%%%%%%%5%%%%%%%%%%%%%%%%%%%%%%%%%%%%%%%%%%%%%%%%%%%%%%%%%%%%%%%%%%%%%%%%%%%%%%
    $c_{tu}^{1}$        &   $ \ccc{}{uu}{ii33} +\frac{1}{3} \ccc{}{uu}{i33i} $ \\   \hline
        %%%%%%%%%%%%%%%%%%%%%%%%%%%%%%%%%%5%%%%%%%%%%%%%%%%%%%%%%%%%%%%%%%%%%%%%%%%%%%%%%%%%%%%%%%%%%%%%%%%%%%%%%
    $c_{Qu}^{8}$         &  $  \ccc{8}{qu}{33ii}$\\     \hline
        %%%%%%%%%%%%%%%%%%%%%%%%%%%%%%%%%%5%%%%%%%%%%%%%%%%%%%%%%%%%%%%%%%%%%%%%%%%%%%%%%%%%%%%%%%%%%%%%%%%%%%%%%
    $c_{Qu}^{1}$     &  $  \ccc{1}{qu}{33ii}$  \\     \hline
        %%%%%%%%%%%%%%%%%%%%%%%%%%%%%%%%%%5%%%%%%%%%%%%%%%%%%%%%%%%%%%%%%%%%%%%%%%%%%%%%%%%%%%%%%%%%%%%%%%%%%%%%%
    $c_{td}^{8}$        &   $\ccc{8}{ud}{33jj}$ \\    \hline
        %%%%%%%%%%%%%%%%%%%%%%%%%%%%%%%%%%5%%%%%%%%%%%%%%%%%%%%%%%%%%%%%%%%%%%%%%%%%%%%%%%%%%%%%%%%%%%%%%%%%%%%%%
    $c_{td}^{1}$          &  $ \ccc{1}{ud}{33jj}$ \\     \hline
        %%%%%%%%%%%%%%%%%%%%%%%%%%%%%%%%%%5%%%%%%%%%%%%%%%%%%%%%%%%%%%%%%%%%%%%%%%%%%%%%%%%%%%%%%%%%%%%%%%%%%%%%%
    $c_{Qd}^{8}$        &   $ \ccc{8}{qd}{33jj}$ \\     \hline
        %%%%%%%%%%%%%%%%%%%%%%%%%%%%%%%%%%5%%%%%%%%%%%%%%%%%%%%%%%%%%%%%%%%%%%%%%%%%%%%%%%%%%%%%%%%%%%%%%%%%%%%%%
    $c_{Qd}^{1}$         &   $ \ccc{1}{qd}{33jj}$\\
        %%%%%%%%%%%%%%%%%%%%%%%%%%%%%%%%%%5%%%%%%%%%%%%%%%%%%%%%%%%%%%%%%%%%%%%%%%%%%%%%%%%%%%%%%%%%%%%%%%%%%%%%%
         \bottomrule
\end{tabular}
}
\end{center}
  \caption{Upper table:  definition of the two-fermion dimension-six
    SMEFT operators relevant for this analysis.
    These operators modify the interactions of the third-generation
    quarks.
    We also indicate the notation for the associated Wilson coefficients; those
    in brackets are not degrees of freedom entering the fit.
    Middle table: the two additional degrees of freedom
    used in the fit involving two-fermion operators, defined in terms
    of the coefficients of the upper table.
    Bottom table:
    the four-fermion degrees of freedom considered here,
    expressed in terms of the corresponding four-fermion Wilson coefficients
    of dimension-six SMEFT operators in the Warsaw basis.
    \label{tab:ops}}
\end{table}
