# Supplementary material for: Precision phenomenology of the PDF-BSM interplay
Source: arXiv:2503.02827 source file (2025-03-04)
Supplement: Supplementary file 19 [file tab_chi2_weighted.tex]

\begin{table}[t]
        \tiny
        \centering
        \begin{tabular}{lc|c|c|c|c|c|}
                \toprule
       & & \multicolumn{2}{c}{SM} & \multicolumn{2}{c}{$W=8\cdot 10^{-5}$}\\
          \midrule
       Dataset  & $n_{\rm dat}$ & $\chi^2$  & $\chi^2$ (weighted) & $\chi^2$ & $\chi^2$ (weighted) \\
          \midrule
           E866 (NuSea) & 89 & 0.80 & 0.81 & 0.98 & 1.14 \\
           D0  $W$ muon asymmetry & 9 & 2.38 & 2.76 & 3.05  & 3.82\\
         ATLAS \(W, Z\) 7 TeV (${\cal L}=4.6\,{\rm fb}^{-1}$) central & 46 & 0.81 & 0.82 & 0.82 & 0.82\\
         ATLAS \(W, Z\) 7 TeV (${\cal L}=4.6\,{\rm fb}^{-1}$) forward & 15 & 1.82 & 1.80 & 1.81 & 1.80 \\
%                \midrule
%                ATLAS high-mass DY 7 TeV (${\cal L}=49\,{\rm fb}^{-1}$)& 13 & 0.85  & 0.85 & 0.87 & 0.84 \\
%                ATLAS high-mass DY 2D 8 TeV & 46 & 0.86 & 0.85 & 0.88 & 0.86 \\
%                CMS high-mass DY 2D 7 TeV & 117 & 0.90 & 0.90 & 0.91 & 0.90 \\
%                CMS high-mass DY 8 TeV & 41 & 0.84 & 0.84 & 0.85 & 0.84 \\
%                CMS high-mass DY 13 TeV & 43 & 1.12 & 1.12 &1.13 & 1.13 \\
                \midrule
                HL-LHC NC \(e\)& 16 & 1.98 & 1.79 & 2.21 & 1.83 \\
                HL-LHC NC \(\mu\)& 16 & 1.10 & 1.04 & 1.17 & 1.05\\
                HL-LHC CC \(e\)& 12 & 0.75 & 0.74 & 1.14 & 0.77\\
                HL-LHC CC \(\mu\)& 12 & 0.65 & 0.64 & 1.16 & 0.63  \\
                \midrule
                \textbf{Total} & \textbf{4771} & \textbf{0.97} & -1.41 & \textbf{0.96} &-1.89 \\
                \bottomrule
        \end{tabular}
        \caption{\label{tab:chi2weighted} Values of the \(\chi^2\) per data point  in the baseline and in the $\hat{W}=8\cdot 10^{-5}$ contaminated fit 
        in the regular fit and in a weighted fit in which high-mass Drell-Yan data are given a larger weight according to Eq.~\eqref{eq:wgts}.}
\end{table}
