# Supplementary material for: Precision phenomenology of the PDF-BSM interplay
Source: arXiv:2503.02827 source file (2025-03-04)
Supplement: Supplementary file 22 [file app-notation.tex]

\section{Notation}
\label{app-notation}

In QCD the $\beta$ function is given by
\begin{equation}
\label{eq:beta}
\beta(\alpha_S) = -b \alpha_S^2 (1 + b^{\prime}\alpha_S + b^{\prime \prime} \alpha_S^2 + \mathcal{O}(\alpha_S^3)), 
\end{equation}
where the coefficients are given by 
\begin{align}
    b &= \frac{33-2 n_f}{12 \pi}, \\
    b^{\prime} &= \frac{153 - 19 n_f}{2 \pi (33 -2 n_f)}, \\
    b^{\prime\prime} &= \frac{77139 - 15099 n_f + 325 n_f^2}{288 \pi^2 (33 - 2 n_f)},   
\end{align}
where $n_f$ is the number of active flavours at the energy scale $\mu$, and the first, second, and third terms on the right-hand side of Eq. (\ref{eq:beta}) represent respectively the $1$-loop, $2$-loop, and $3$-loop corrections.

The leading-order QCD splitting functions are given by
\begin{equation}
\label{eq:sm_P}
\begin{aligned}
    P_{qq}(z) &= C_F \left(\frac{1+z^2}{(1-z)_+} + \frac{3}{2}\delta(1-z) \right), \\
    P_{gq}(z) &= C_F \left(\frac{1+(1-z)^2}{z} \right), \\
    P_{qg}(z) &= T_F (z^2 + (1-z)^2),\\
    P_{gg}(z) &= 2 C_A \left( \frac{z}{(1-z)_+} + \frac{1-z}{z} + z(1-z)\right) + \left( \frac{11 C_A}{6} - \frac{2}{3}T_F n_f  \right) \delta(1-z), 
\end{aligned}
\end{equation}
where $C_F = 4/3$, $T_F=1/2$, $C_A = 3$, and the plus distribution for any smooth function $f(x)$ satisfies 
\begin{equation*}
    \int_{0}^{1} \frac{f(x)}{(1-x)_{+}} dx = \int_{0}^{1} \frac{f(x) - f(1)}{1-x} dx. 
\end{equation*}
