# Supplementary material for: Precision phenomenology of the PDF-BSM interplay
Source: arXiv:2503.02827 source file (2025-03-04)
Supplement: Supplementary file 24 [file app_denoising.tex]

\section{Selection criteria and denoising}
\label{app:denoising}

PySR has three selection criteria options:
\begin{itemize}
    \item \texttt{accuracy}: selects the candidate model with the lowest loss.
    \item \texttt{best}: selects the candidate model with the highest score among expressions with a loss better than at least $1.5x$ the most accurate model. This is the default criterion.
    \item \texttt{score}: selects the candidate model with the highest score, defined as the negated derivative of the log-loss with respect to complexity.
\end{itemize}

Additionally, PySR has a denoising feature which can perform an optional preprocessing step that refines the input data using a Gaussian process with an adaptable kernel. This kernel is a composite of a Gaussian function for smoothing, a white noise component to address inherent noise, and a constant kernel to adjust the mean of the Gaussian process. The Gaussian process then provides denoised target values for each data point, which PySR then fits.

We can use the events of subsection \ref{subsec:l1} to evaluate the results that we obtain with the denoising feature. We show the equations that we obtain with PySR, according to the denoising options and the three  selection criteria, in tables \ref{tab:10bins}, \ref{tab:30bins}, and \ref{tab:100bins}, for 10, 30, and 100 bins, respectively. We see that, in general, the denoising Gaussian process leads to more convolved equations that miss the real distribution. Not using the denoising tends to lead to better performance. It is worth noting, however, that PySR can deal with noisy data in different ways. One alternative is to use a weighted loss that accounts for the uncertainty in each target value. 

\begin{table}[h]
\begin{center}
\begin{tabular}{@{}cl|l|l@{}}
\toprule
Denoise & \multicolumn{1}{c}{Accuracy} & \multicolumn{1}{c}{Best} & \multicolumn{1}{c}{Score} \\
\midrule
True & 
\begin{minipage}[t]{0.25\columnwidth}$0.0007090032 \cdot x_{0} + 9090.917$\end{minipage} & 
\begin{minipage}[t]{0.25\columnwidth}$9090.844 \cdot x_{0} \cdot (9.63109 \cdot 10^{-5} - 7.7957055 \cdot 10^{-5} \cdot x_{0}) \cdot (x_{0} - 0.22291435) + 9090.844$\end{minipage} & 
\begin{minipage}[t]{0.25\columnwidth}$0.20396256 \cdot x_{0} + 9090.812$\end{minipage} \\
\noalign{\smallskip} \hline \noalign{\smallskip}
False & 
\begin{minipage}[t]{0.25\columnwidth}$x_{0}^{2} \cdot (296.52358194355 \cdot x_{0}^{4} + 7046.0674) + 7613.42$\end{minipage} & 
\begin{minipage}[t]{0.25\columnwidth}$7250.1396 \cdot x_{0}^{2} + 7589.319$\end{minipage} & 
\begin{minipage}[t]{0.25\columnwidth}$7250.1396 \cdot x_{0}^{2} + 7589.319$\end{minipage} \\
\bottomrule
\end{tabular}
\caption{SR results for 10 bins.}
\label{tab:10bins}
\end{center}
\end{table}

\begin{table}[h]
\begin{center}
\begin{tabular}{@{}cc|c|c@{}}
\toprule
Denoise & Accuracy & Best & Score \\
\midrule
True & 
\begin{minipage}[t]{0.25\columnwidth}$-0.21235736(x_{0}-1.1249065)(2x_{0}-1.1303912)(2x_{0}+0.2443421) + 3225.8237$\end{minipage} & 
\begin{minipage}[t]{0.25\columnwidth}$0.024268737x_{0}^{2} + 3225.7983$\end{minipage} & 
\begin{minipage}[t]{0.25\columnwidth}$x_{0}^{2}(-0.86325264x_{0}^{2} + x_{0}) + 3225.7295$\end{minipage} \\
\noalign{\smallskip} \hline \noalign{\smallskip}
False & 
\begin{minipage}[t]{0.25\columnwidth}$x_{0}^{2}(123.43398x_{0}^{4}+2326.98053420264)+2538.3494$\end{minipage} & 
\begin{minipage}[t]{0.25\columnwidth}$2417.7627x_{0}^{2} + 2527.635$\end{minipage} & 
\begin{minipage}[t]{0.25\columnwidth}$2415.3643x_{0} + 2125.6453$\end{minipage} \\
\bottomrule
\end{tabular}
\caption{SR results for 30 bins.}
\label{tab:30bins}
\end{center}
\end{table}

\begin{table}[h]
\begin{center}
\begin{tabular}{@{}cc|c|c@{}}
\toprule
Denoise & Accuracy & Best & Score \\
\midrule
True & 
\begin{minipage}[t]{0.25\columnwidth}$x_{0}^{2}(-1.615747x_{0}^{2}+2x_{0}-0.081652954)+995.048$\end{minipage} & 
\begin{minipage}[t]{0.25\columnwidth}$x_{0}(-0.46552044x_{0}^{4}+x_{0}-0.24463812)+995.06415$\end{minipage} & 
\begin{minipage}[t]{0.25\columnwidth}$995.1925$\end{minipage} \\
\noalign{\smallskip} \hline \noalign{\smallskip}
False & 
\begin{minipage}[t]{0.25\columnwidth}$x_{0}(207.340216x_{0}+428.81232)+109.830989048+750.30175$\end{minipage} & 
\begin{minipage}[t]{0.25\columnwidth}$726.08685x_{0}^{2}+757.9762$\end{minipage} & 
\begin{minipage}[t]{0.25\columnwidth}$725.2477x_{0}+637.3749$\end{minipage} \\
\bottomrule
\end{tabular}
\caption{SR results for 100 bins.}
\label{tab:100bins}
\end{center}
\end{table}

The denoising option proved to be effective just to fit the level 1 distribution with a $(1 + \cos^2 \theta)^{-1}$ reweighting to find the overall constant, as shown in Tab. \ref{tab:const}. With denoising, any selection criterion gives the correct constant answer. On the other hand, if the denoising is not applied PySR finds equations that are more expressive than the real law of Nature.

\begin{table}[h]
\begin{center}
\begin{tabular}{@{}l|c|c|c@{}}
\toprule
Denoise & Accuracy & Best & Score \\
\midrule
True & 
$6833.678$ & 
$6833.678$ & 
$6833.678$ \\
\noalign{\smallskip} \hline \noalign{\smallskip}
False & 
\begin{minipage}[t]{0.25\columnwidth}
$x_{0}^{2}(661.2393x_{0} - 706.5968)(x_{0}^{2} + x_{0}) + 7593.010$
\end{minipage} & 
\begin{minipage}[t]{0.25\columnwidth}
$7614.049 - 194.01741x_{0}$
\end{minipage} & 
\begin{minipage}[t]{0.25\columnwidth}
$7614.0547 - 194.02724x_{0}$
\end{minipage} \\
\bottomrule
\end{tabular}
\caption{SR equations with denoising for the reweighted distribution.}
\label{tab:const}
\end{center}
\end{table}

The SR results are consistent even if we change the number of events of the dataset ($10^4$ or $10^5$, for example) and obtain different levels of statistical uncertainty.

It is reassuring that, even if we do not input our knowledge of the Natural law by reweighting the level 1 distribution, PySR is still clever enough to find the correct functional form in spite of the noise in the data.
