# Supplementary material for: Precision phenomenology of the PDF-BSM interplay
Source: arXiv:2503.02827 source file (2025-03-04)
Supplement: Supplementary file 27 [file chi2_pdfs.tex]

%%%%%%%%%%%%%%%%%%%%%%%%%%%%%%%%%%%%%%%%%%%%%%%%%%%%%%%%%%%%%%%%%%%%%%
\begin{table}[htbp]
  \begin{center}
  
%\scriptsize
\tiny
\begin{tabular}{ l | c| C{1.2cm} | C{1.2cm} | C{1.0cm} | C{1.2cm} | C{1.2cm} | C{1.2cm} }
 \toprule
 \multirow{3}{*}{Dataset}    & \multirow{3}{*}{$n_{\rm dat}$}   &  \multicolumn{6}{c}{$\chi^2/n_{\rm dat}$}  \\[1.5ex]
 &   & \multicolumn{3}{c|}{\bf SM-PDF fits} & \multicolumn{2}{c|}{\bf Fixed-PDF EFT fits}   & {\bf SMEFT-PDFs}    \\
  &   & NNPDF4.0 (no top)  & NNPDF4.0 & Fit H & NNPDF4.0 (no top) & Fit H & Joint fit   \\
 \midrule
 \midrule
 SLAC      & 67   & 0.768   & 0.758 & 0.753 & 0.768 & 0.753  & 0.761  \\
 BCDMS   & 581 &  	1.265  & 1.247 & 1.251 & 1.265  & 1.251  & 1.245   \\
 NMC       & 325 & 1.298   & 1.306 & 1.304  & 1.298  & 1.304  & 1.292    \\
 CHORUS  & 832 & 0.899    & 0.900 & 0.901  & 0.899  & 0.901  & 0.898     \\
  NuTeV     & 76  & 0.398 & 0.425  & 0.423 & 0.398  & 0.423  & 0.393    \\
 HERA  & 1208 & 1.204  & 1.203 & 1.204  & 1.204  & 1.204  & 1.200    \\
 \midrule
     {\bf Total DIS}  & {\bf 3089} &  {\bf 1.122 }  & {\bf 1.119 } & {\bf 1.119 } & {\bf 1.122 } & {\bf 1.119 } & {\bf 1.114 } \\
     \midrule
     \midrule
 E886    $\sigma^d_{\rm DY}/\sigma^p_{\rm DY}$ & 15  & 0.527    & 0.524  & 0.536  & 0.527 & 0.536   & 0.544   \\
 E886    $\sigma^p_{\rm DY}$                               & 89  & 1.566  & 1.559  & 1.615  & 1.566 & 1.615  & 1.602   \\
 E605   $\sigma^p_{\rm DY}$                                & 85  & 0.456   & 0.456  & 0.460 & 0.456  & 0.460  & 0.464    \\
 E906   $\sigma^d_{\rm DY}/\sigma^p_{\rm DY}$ &  6  &  0.827   &    0.885  & 0.886   & 0.827 & 0.886  &  0.955    \\
\midrule
{\bf Total fixed-target DY} & {\bf 195} & {\bf 0.981 } & {\bf 0.979 }   & {\bf 1.008 } & {\bf 0.981} & {\bf 1.008 } & {\bf 1.006 }  \\
 \midrule
 \midrule
 CDF    $d\sigma_Z/dy_Z$                                    & 28 &  1.234  & 1.280  &  1.275 & 1.234  & 1.275  & 1.188    \\
 D0     $d\sigma_Z/dy_Z$                                     & 28 &   0.637  & 0.644 &  0.640 & 0.637  & 0.640 & 0.632   \\
 D0    	$W\to \mu \nu$ asy.                       & 9  &   1.958 & 1.929 & 1.905  & 1.958  & 1.905 & 1.641     \\
 \midrule
 ATLAS low-mass DY 7 TeV               & 6 &  0.875  & 0.879 & 0.883  & 0.875  & 0.883 & 0.888    \\
 ATLAS high-mass DY 7 TeV               & 5 & 1.694 & 1.691 & 1.661 & 1.694  & 1.661 & 1.629  \\
 ATLAS $W, Z$ 7 TeV ($\mathcal{L} = 35$ pb${}^{-1}$) & 30   &  1.000 & 0.988 & 1.000 & 1.000 & 1.000  & 0.991    \\
 ATLAS  $W,Z$ 7 TeV ($\mathcal{L} = 4.6$ fb${}^{-1}$) & 61  & 1.689 & 1.686  & 1.685 & 1.685  & 1.685 & 1.599    \\
ATLAS low-mass DY 2D 8 TeV            & 60 & 1.203 &1.216 & 1.225 & 1.203  & 1.225 & 1.207   \\
ATLAS high-mass DY 2D 8 TeV           & 48 & 1.123  & 1.110 & 1.118 & 1.123  & 1.118 & 1.147   \\
ATLAS $\sigma_{W,Z}^{\rm tot}$ 13 TeV    & 3 & 0.727 & 0.778  & 0.706 & 0.727 & 0.706 & 0.471 \\
 \midrule
 CMS $W$ electron asymmetry 7 TeV             & 11 & 0.836 & 0.833 & 0.836 & 0.836 & 0.836 & 0.892   \\
CMS $W$ muon asymmetry 7 TeV              & 11 & 1.728 & 1.714 & 1.733 & 1.728  & 1.733 &  1.699  \\
CMS DY 2D 7 TeV                                        & 110 & 1.367 & 1.361 & 1.353 & 1.367 & 1.353 &  1.339 \\
CMS $W$ rapidity 8 TeV                              & 22 & 1.375 & 1.361 & 1.365 & 1.375  & 1.365 & 1.162  \\
 \midrule
 LHCb $Z \rightarrow ee$ 7 TeV                       & 9  &  1.630  & 1.648 & 1.636 & 1.630 & 1.636 & 1.669 \\
 LHCb $Z \rightarrow ee$ 8 TeV                        & 17  & 1.272   & 1.325 & 1.334 & 1.272 &  1.334 & 1.266 \\
 LHCb  $W,Z \rightarrow \mu$  7 TeV                 & 29  &   2.032 &  1.948 & 1.902 & 2.032 & 1.902 & 1.896   \\
 LHCb  $W,Z \rightarrow \mu$   8 TeV                & 30  & 1.494   & 1.426 & 1.417 & 1.494  & 1.417 & 1.386  \\
  LHCb  $Z \rightarrow ee$   13 TeV                & 15  & 1.701 & 1.726  & 1.717  & 1.701  & 1.717 & 1.640   \\
  LHCb  $Z \rightarrow \mu\mu$   13 TeV                & 16  & 0.970 & 0.993 & 0.978  & 0.970  & 0.978 & 0.928   \\
\midrule
{\bf Total inclusive gauge boson production} & {\bf 548} &  {\bf 1.344}  & {\bf 1.339}  & {\bf 1.335}  & {\bf 1.344}  & {\bf 1.335} & {\bf 1.297}    \\
 \midrule
 \midrule
ATLAS $W^{\pm}+$jet 8 TeV                      & 30 & 0.954 & 0.959 & 0.957  & 0.954  & 0.957 & 0.973 \\
ATLAS $Z$ $p_T$ 8 TeV ($p_T, m_{\ell\ell}$)      & 44 & 0.911 & 0.905 & 0.904 & 0.911 & 0.904 & 0.910 \\
ATLAS $Z$ $p_T$ 8 TeV ($p_T, y_Z$)                 & 48 & 0.909 & 0.898 & 0.896 & 0.909 & 0.896 & 0.924\\
ATLAS incl. jets 8 TeV, $R=0.6$                           & 171 & 0.682 & 0.687 & 0.687 & 0.682  & 0.687 & 0.667  \\
ATLAS dijets 7 TeV, $R=0.6$                               & 90 & 2.184  & 2.149  & 2.125  & 2.184 & 2.125 &. 2.177  \\
ATLAS isolated $\gamma$ prod. 13 TeV             & 53 & 0.811  & 0.763 & 0.753 & 0.811  & 0.753 & 0.813  \\
 \midrule
CMS $Z$ $p_T$ 8 TeV                                 & 28 & 1.447 & 1.401 & 1.407  & 1.447 & 1.407 & 1.473  \\
CMS incl. jets 8 TeV                                     & 185 & 1.140 & 1.183 & 1.200 & 1.140  & 1.200 & 1.118   \\
CMS dijets 7 TeV                                          & 54 & 1.788 & 1.810  & 1.809 & 1.788 & 1.809  & 1.800  \\
 \midrule
     {\bf Total jets, $Z$ $p_T$ and isolated photon}                      & {\bf 703} &  {\bf 1.154}  & {\bf 1.157} & {\bf 1.158}  & {\bf 1.154}  & {\bf 1.158}  & {\bf 1.148}  \\
      \midrule
 \midrule
     {\bf Total non-top data}                      & {\bf 4535} & {\bf 1.148}  &  {\bf 1.145} & {\bf 1.146} & {\bf 1.148} & {\bf 1.146} & {\bf 1.137} \\
 \bottomrule
\end{tabular}
\end{center}
  \caption{\small \label{tab:chi2-baseline} The values of the $\chi^2$ per data point (using the experimental
    definition of Eq.~\eqref{eq:chi2exp}) for key PDF and EFT analyses presented in this work.
    For each dataset, we indicate the number of data points $n_{\rm dat}$
    and the the $\chi^2$ values for {\it i)} three SM-PDF fits:
    \nnpdfnotop, \nnpdf,
    and Fit H in Table~\ref{tab:fit_list} (full top quark dataset);
    {\it ii)} two fixed-PDF EFT fits: one based on \nnpdfnotop as input,
    and the other using Fit H as input; and finally  {\it iii)} the outcome
    of the simultaneous SMEFT-PDF determination.
    Here we restrict ourselves to the non-top datasets considered in this
    analysis, the corresponding results for the top quark observables
    are provided in Tables~\ref{tab:chi2-top} and~\ref{tab:chi2-single-top}.
    We also provide the total $\chi^2$ for separate groups of processes as well
    as for the full non-top dataset.
    The $\chi^2$ values for the \nnpdfnotop fit
    and for the fixed-PDF EFT fit based on \nnpdfnotop are identical,
    since the latter uses only top data as input.
    For the same reason, the entries in the columns for the SM-PDF Fit H
    and the fixed-PDF EFT fits based on Fit H are the same.
}
\end{table}
%%%%%%%%%%%%%%%%%%%%%%%%%%%%%%%%%%%%%%%%%%%%%%%%%%%%%%%%%%%%%%%%%%%%%%%%%%
%%%%%%%%%%%%%%%%%%%%%%%%%%%%%%%%%%%%%%%%%%%%%%%%%%%%%%%%%%%%%%%%%%%%%%%%%%%%%%%%
