# Supplementary material for: Precision phenomenology of the PDF-BSM interplay
Source: arXiv:2503.02827 source file (2025-03-04)
Supplement: Supplementary file 28 [file chi2_pdfs_single_top.tex]

\begin{table}[htbp]
  \begin{center}
  
%\scriptsize
    \tiny
\begin{tabular}{ l | c| C{1.2cm} | C{1.2cm} | C{1.0cm} | C{1.2cm} | C{1.2cm} | C{1.5cm} }
 \toprule
 \multirow{3}{*}{Dataset}    & \multirow{3}{*}{$n_{\rm dat}$}   &  \multicolumn{6}{c}{$\chi^2/n_{\rm dat}$}  \\[1.5ex]
 &   & \multicolumn{3}{c|}{\bf SM-PDF fits} & \multicolumn{2}{c|}{\bf Fixed-PDF EFT fits}   & {\bf SMEFT-PDFs}    \\
  &   & NNPDF4.0 (no top)  & NNPDF4.0 & Fit H & NNPDF4.0 (no top) & Fit H & Joint fit   \\
 \midrule
 \midrule
     ATLAS $t$-channel $\sigma(t)$, 7 TeV & 1 & \textit{0.785} & \textit{0.756} & 0.757 & 0.179 & 0.135 & 0.155  \\
    ATLAS $t$-channel $\sigma(\bar{t})$, 7 TeV & 1 & \textit{0.304}  & \textit{0.296} & 0.282 & 0.003 & 0.005 & 0.004  \\
    ATLAS $t$-channel $1/\sigma d\sigma(tq)/dy_t$, 7 TeV & 3 & \textit{0.909} & 0.959 & 0.971 & 0.885 & 0.946 & 0.900  \\
     ATLAS $t$-channel $1/\sigma d\sigma(\bar{t}q)/dy_{\bar{t}}$, 7 TeV & 3 & \textit{0.061}  & 0.062 & 0.062 & 0.061 & 0.063 & 0.062  \\
     ATLAS $t$-channel $\sigma(t)$, 8 TeV & 1 & \textit{0.795}  & \textit{0.739} & 0.739 & 0.000 & 0.017 & 0.007 \\
     ATLAS $t$-channel $\sigma(\bar{t})$, 8 TeV & 1 & \textit{2.314} & \textit{2.277}  & 2.221 & 0.379 & 0.337 & 0.356  \\
    ATLAS $t$-channel $1/\sigma d\sigma(tq)/dy_t$, 8 TeV & 3 & \textit{0.288} & 0.246 & 0.241 & 0.290 & 0.245 & 0.283  \\
     ATLAS $t$-channel $1/\sigma d\sigma(\bar{t}q)/dy_{\bar{t}}$, 8 TeV & 3 & \textit{0.196} & 0.190 & 0.187 & 0.198 & 0.189 & 0.192  \\
     ATLAS $s$-channel $\sigma(t + \bar{t})$, 8 TeV & 1 & \textit{0.211} & \textit{0.203} & 0.216 & 0.000 & 0.000 & 0.000  \\
    ATLAS $t$-channel $\sigma(t)$, 13 TeV & 1 & \textit{0.738} & \textit{0.722} & 0.720 & 0.261 & 0.224 & 0.235  \\
    ATLAS $t$-channel $\sigma(\bar{t})$, 13 TeV & 1 & \textit{0.400} & \textit{0.393} & 0.384 & 0.057 & 0.050 & 0.051  \\
     ATLAS $s$-channel $\sigma(t + \bar{t})$, 13 TeV & 1 & \textit{0.700} & \textit{0.688} & 0.703 & 0.127 & 0.138 & 0.118  \\
    \midrule
    CMS $t$-channel $\sigma(t) + \sigma(\bar{t})$, 7 TeV & 1 & \textit{0.765}  & 0.729  & 0.719 & 0.010 & 0.001 & 0.004  \\
    CMS $t$-channel $\sigma(t)$, 8 TeV & 1 & \textit{0.010} & \textit{0.006} & 0.005 & 0.487 & 0.628 & 0.566  \\
    CMS $t$-channel $\sigma(\bar{t})$, 8 TeV & 1 & \textit{0.079} & \textit{0.084} & 0.092 & 0.886 & 0.934  & 0.911 \\
    CMS $s$-channel $\sigma(t + \bar{t})$, 8 TeV & 1 & \textit{1.108}  & \textit{1.112} & 1.105 & 1.348 & 1.338 & 1.350 \\
    CMS $t$-channel $\sigma(t)$, 13 TeV & 1 & \textit{0.904} & \textit{0.883} & 0.880 & 0.281 & 0.235 & 0.248  \\
    CMS $t$-channel $\sigma(\bar{t})$, 13 TeV & 1 & \textit{0.136} & \textit{0.132} & 0.125 & 0.010 & 0.014 & 0.013 \\
   CMS $t$-channel $1/\sigma d\sigma/d|y^{(t)}|$, 13 TeV & 4 & \textit{0.412} & \textit{0.387} & 0.383 & 0.405 & 0.378 & 0.396  \\
       \midrule
   {\bf Total single top}  & {\bf 30}  & {\bf 0.509 }  &  {\bf 0.498 } & {\bf 0.495 } & {\bf 0.332 } & {\bf 0.330 } & {\bf 0.331 }  \\
     \midrule
     \midrule
    ATLAS $\sigma(tW)$, dilepton, 8 TeV & 1 & \textit{0.510} & \textit{0.529} & 0.538 & 0.144  & 0.168 & 0.167 \\
    ATLAS $\sigma(tW)$, single-lepton, 8 TeV & 1 & \textit{0.695} & \textit{0.708} & 0.713 & 0.428 & 0.449 & 0.448  \\
    ATLAS $\sigma(tW)$, dilepton, 13 TeV & 1 & \textit{1.150} & \textit{1.149} & 1.148 & 0.840 & 0.847 & 0.849  \\
    ATLAS $\sigma_{\text{fid}}(tZj)$, dilepton, 13 TeV & 1 & \textit{0.115} & \textit{0.115} & \textit{0.115} & 0.871 & 0.611 & 0.795  \\
    \midrule
    CMS $\sigma(tW)$, dilepton, 8 TeV & 1 & \textit{0.359} & \textit{0.371} & 0.376 & 0.134 & 0.150 & 0.149 \\
    CMS $\sigma(tW)$, dilepton, 13 TeV & 1 & \textit{0.434} & \textit{0.437} & 0.438 & 1.612 & 1.573 & 1.563 \\
    CMS $\sigma_{\text{fid}}(tZj)$, dilepton, 13 TeV & 1 & \textit{1.041} & \textit{1.041} & \textit{1.041} & 0.279 & 0.427 & 0.316  \\
    CMS $d\sigma_{\text{fid}}(tZj)/dp_T^{t}$, dilepton, 13 TeV & 3 & \textit{0.362} & \textit{0.362} & \textit{0.362} & 0.130 & 0.156 & 0.134  \\
   CMS $\sigma(tW)$, single-lepton, 13 TeV & 1 & \textit{2.837} & \textit{2.833} & 2.832 & 1.817 & 1.839 & 1.846  \\
    \midrule
   {\bf Total associated single top}  & {\bf 11}  & {\bf 0.748 }  & {\bf 0.752 } &  {\bf 0.753 }  & {\bf 0.592 } & {\bf 0.594 } & {\bf 0.594 } \\
     \midrule
     \midrule
   {\bf Total top}  & {\bf 175}  & {\bf 1.370}   & {\bf 1.139} & {\bf 1.102} & {\bf 0.868} & {\bf 0.839} & {\bf 0.848}    \\
     \midrule
     \midrule
     {\bf Total dataset}   &  {\bf 4710} & {\bf 1.156}  & {\bf 1.145} & {\bf 1.144} & {\bf 1.138} & {\bf 1.135} & {\bf 1.126}  \\
 \bottomrule
\end{tabular}
\end{center}
  \caption{\small \label{tab:chi2-single-top}
     Same as Table~\ref{tab:chi2-top} now
    for the  inclusive and associated single-top production datasets.
    Values in italics indicate datasets 
    that do not enter the corresponding fits: for those processes,
    we evaluate a posteriori the physical observables and the associated
    $\chi^2$ values using the resulting PDFs from the fit.
    The last row indicates the total values adding together the non-top
    and top data contributions to the $\chi^2$,
    and the next-to-last row the total top quark contribution.
}
\end{table}
%%%%%%%%%%%%%%%%%%%%%%%%%%%%%%%%%%%%%%%%%%%%%%%%%%%%%%%%%%%%%%%%%%%%%%%%%%
%%%%%%%%%%%%%%%%%%%%%%%%%%%%%%%%%%%%%%%%%%%%%%%%%%%%%%%%%%%%%%%%%%%%%%%%%%%%%%%%
