# Supplementary material for: Precision phenomenology of the PDF-BSM interplay
Source: arXiv:2503.02827 source file (2025-03-04)
Supplement: Supplementary file 29 [file chi2_pdfs_top.tex]

%%%%%%%%%%%%%%%%%%%%%%%%%%%%%%%%%%%%%%%%%%%%%%%%%%%%%%%%%%%%%%%%%%%%%%
\begin{table}[htbp]
  \begin{center}
  
%\scriptsize
  \tiny
\begin{tabular}{ l | c| C{1.2cm} | C{1.2cm} | C{0.8cm} | C{1.2cm} | C{1.0cm} | C{1.2cm} }
 \toprule
 \multirow{3}{*}{Dataset}    & \multirow{3}{*}{$n_{\rm dat}$}   &  \multicolumn{6}{c}{$\chi^2/n_{\rm dat}$}  \\[1.5ex]
 &   & \multicolumn{3}{c|}{\bf SM-PDF fits} & \multicolumn{2}{c|}{\bf Fixed-PDF EFT fits}   & {\bf SMEFT-PDFs}    \\
  &   & NNPDF4.0 (no top)  & NNPDF4.0 & Fit H & NNPDF4.0 (no top) & Fit H & Joint fit   \\
 \midrule
 \midrule
    ATLAS $\sigma(t\bar{t})$, dilepton, 7 TeV    & 1    &   \textit{4.100}  & 4.540 & 4.599 & 1.733 & 1.824 & 1.974     \\
    ATLAS $\sigma(t\bar{t})$, dilepton, 8 TeV & 1 & \textit{0.005} & 0.021 & 0.023 & 0.405 & 0.382 & 0.307 \\
    ATLAS $1/\sigma d\sigma/dm_{t\bar{t}}$, dilepton, 8 TeV & 5 & \textit{0.262} & \textit{0.284} & 0.291 & 0.305 & 0.309 & 0.310  \\
    ATLAS $\sigma(t\bar{t})$, $\ell+$jets, 8 TeV & 1 & \textit{0.218} & \textit{0.270} & 0.277 & 0.002 & 0.001  & 0.000  \\
    ATLAS $1/\sigma d\sigma/d|y_t|$, $\ell+$jets, 8 TeV & 4 & \textit{6.266} & 3.219 & 2.827 & 1.178 & 1.021 & 1.144 \\
    ATLAS $1/\sigma d\sigma/d|y_{t\bar{t}}|$, $\ell+$jets, 8 TeV & 4 & \textit{7.978} & 3.725 & 3.332 & 2.883 & 2.105 & 2.646  \\
    ATLAS $\sigma(t\bar{t})$, dilepton, 13 TeV           & 1    &  \textit{1.388}  & \textit{1.397}  & 1.374 & 0.004 & 0.004 & 0.002    \\
    ATLAS $\sigma(t\bar{t})$, hadronic, 13 TeV         & 1    & \textit{0.231}   &  \textit{0.231} & 0.230 & 0.082 & 0.082  & 0.092    \\
    ATLAS $1/\sigma d^2\sigma/d|y_{t\bar{t}}|dm_{t\bar{t}}$, hadronic, 13 TeV & 10 & \textit{2.276}  & \textit{2.007}  & 1.928 & 1.915 & 1.824 & 1.857  \\
    ATLAS $\sigma(t\bar{t})$, $\ell+$jets, 13 TeV & 1 & \textit{0.489} & 0.492 & 0.485 & 0.004 & 0.004 & 0.013 \\
    ATLAS $1/\sigma d\sigma/dm_{t\bar{t}}$, $\ell+$jets, 13 TeV & 8 & \textit{1.607} & \textit{1.788}  & 1.835 & 2.087 & 2.072 & 2.090  \\
    \midrule
    CMS $\sigma(t\bar{t})$, combined, 5 TeV & 1 & \textit{0.442}  & 0.542 & 0.555 & 0.211 & 0.236 & 0.239  \\
    CMS $\sigma(t\bar{t})$, combined, 7 TeV & 1 & \textit{0.795} & 1.032 & 1.065 & 0.004 & 0.010 & 0.027  \\
    CMS $\sigma(t\bar{t})$, combined, 8 TeV & 1 & \textit{0.170} & 0.247 & 0.258 & 0.174 & 0.156 & 0.103  \\
    CMS $1/\sigma d^2\sigma/d|y_{t\bar{t}}|dm_{t\bar{t}}$, dilepton, 8 TeV & 16 & \textit{1.094}  & \textit{0.994} & 0.963  & 0.519 & 0.580 & 0.514  \\
    CMS $1/\sigma d\sigma/d|y_{t\bar{t}}|$, $\ell+$jets, 8 TeV & 9 & \textit{2.127} &1.245 & 1.131 & 0.928 & 0.995 & 0.935  \\
    CMS $\sigma(t\bar{t})$, dilepton, 13 TeV & 1 & \textit{0.064}  & 0.063 & 0.066 & 0.680 & 0.680 & 0.600  \\
    CMS $1/\sigma d\sigma/dm_{t\bar{t}}$, dilepton, 13 TeV & 5 & \textit{2.760}  & 2.550 & 2.485 & 2.246 & 2.232 & 2.194  \\
    CMS $\sigma(t\bar{t})$, $\ell+$jets, 13 TeV & 1 & \textit{0.230} & \textit{0.227} & 0.234 & 2.153 & 2.155  & 1.907  \\
    CMS $1/\sigma d\sigma/dm_{t\bar{t}}$, $\ell+$jets, 13 TeV & 14 & \textit{1.829}  & \textit{1.481} & 1.393 & 0.962 & 0.911 & 0.912  \\
    \midrule
    ATLAS charge asymmetry, 8 TeV & 1 & \textit{0.679}  & \textit{0.678} & 0.675 & 0.567 & 0.587 & 0.571 \\
    ATLAS charge asymmetry, 13 TeV & 5 & \textit{1.012} & \textit{0.997} & 0.989 & 0.872 & 0.786 & 0.836 \\
    CMS charge asymmetry, 8 TeV & 3 & \textit{0.052} & \textit{0.052} & 0.053 & 0.072 & 0.069  & 0.071\\
    CMS charge asymmetry, 13 TeV & 3 & \textit{0.277} & \textit{0.283} & 0.286 & 0.443 & 0.510 & 0.451  \\
    ATLAS \& CMS combined charge asy., 8 TeV & 6 & \textit{0.603}  &\textit{0.602} & 0.602 & 0.646 & 0.659 & 0.651  \\
    \midrule
    ATLAS $W$-hel., 13 TeV & 2 & \textit{0.370} & \textit{0.370} & \textit{0.370} & 0.037 & 0.037 & 0.038   \\
    ATLAS \& CMS combined $W$-hel., 8 TeV & 2 & \textit{1.046} & \textit{1.046} & \textit{1.046} & 0.853 & 0.853 & 0.854  \\
       \midrule
   {\bf Total inclusive $t\bar{t}$}  & {\bf 108}  &  {\bf 1.700 } &  {\bf 1.328 } & {\bf 1.271 } & {\bf 1.032 } & {\bf 0.994} & {\bf 1.002 }  \\
     \midrule
     \midrule
    ATLAS $\sigma(t\bar{t}Z)$, 8 TeV & 1 & \textit{0.264}  &   \textit{0.232}  & 0.235 & 1.331 & 1.161 & 1.258 \\
    ATLAS $\sigma(t\bar{t}W)$, 8 TeV & 1 &  \textit{2.461} &  \textit{2.482} & 2.430 & 0.751 & 0.708 & 0.722   \\
    ATLAS $\sigma(t\bar{t}Z)$, 13 TeV & 1 &  \textit{0.702} &  \textit{0.747} & 0.742 & 0.001 & 0.000 & 0.000  \\
    ATLAS $1/\sigma d\sigma(t\bar{t}Z)/dp_T^Z$, 13 TeV & 5 &  \textit{1.961}  &  \textit{1.940} & 1.933 & 1.870 & 1.840 & 1.860  \\
    ATLAS $\sigma(t\bar{t}W)$, 13 TeV & 1 &  \textit{1.436} &  \textit{1.456} & 1.417 & 0.000 & 0.002 & 0.000 \\
    \midrule
    ATLAS $\sigma(t\bar{t}\gamma)$, 8 TeV & 1 & \textit{0.426} & \textit{0.426} & \textit{0.426} & 0.037 & 0.009 & 0.034  \\
    \midrule
    ATLAS $\sigma(t\bar{t}t\bar{t})$, multi-lepton, 13 TeV & 1 & \textit{3.655} & \textit{3.655} & \textit{3.655} & 4.289 & 3.784 & 4.145  \\
    ATLAS $\sigma(t\bar{t}t\bar{t})$, single lepton, 13 TeV & 1 & \textit{0.872} & \textit{0.872} & \textit{0.872} & 0.997 & 0.898 & 0.969  \\
    ATLAS $\sigma(t\bar{t}b\bar{b})$, $\ell+$jets, 13 TeV & 1 & \textit{2.062} & \textit{2.062} & \textit{2.062} & 1.093 & 1.316 & 1.152  \\
       \midrule
    CMS $\sigma(t\bar{t}Z)$, 8 TeV & 1 &  \textit{0.432}  &  \textit{0.470} & 0.466 & 0.005 & 0.020 & 0.010 \\
    CMS $\sigma(t\bar{t}W)$, 8 TeV & 1 &  \textit{2.281}  &  \textit{2.298} & 2.255 & 0.808 & 0.770 & 0.783  \\
    CMS $\sigma(t\bar{t}Z)$, 13 TeV & 1 &  \textit{1.185}  &  \textit{1.238} & 1.233 & 0.085 & 0.113 & 0.110 \\
    CMS $1/\sigma d\sigma(t\bar{t}Z)/dp_T^Z$, 13 TeV & 3 &  \textit{0.628}  &  \textit{0.598} & 0.590 & 0.936 & 0.756 & 0.898 \\
    CMS $\sigma(t\bar{t}W)$, 13 TeV & 1 &  \textit{0.667} &  \textit{0.682} & 0.652 & 0.297 & 0.329 & 0.307  \\
    \midrule
    CMS $\sigma(t\bar{t}\gamma)$, 8 TeV & 1 & \textit{0.508} & \textit{0.508} & \textit{0.508} & 0.022 & 0.045 & 0.024 \\
    \midrule
    CMS $\sigma(t\bar{t}t\bar{t})$, multi-lepton, 13 TeV & 1 & \textit{0.027} & \textit{0.027} & \textit{0.027} & 0.124 & 0.041 & 0.096  \\
    CMS $\sigma(t\bar{t}t\bar{t})$, single lepton, 13 TeV & 1 & \textit{0.231} & \textit{0.231} & \textit{0.231} & 0.262 & 0.238 & 0.255 \\
    CMS $\sigma(t\bar{t}b\bar{b})$, all-jet, 13 TeV & 1 & \textit{1.878} & \textit{1.878} & \textit{1.878} & 1.334 & 1.466 & 1.369  \\
    CMS $\sigma(t\bar{t}b\bar{b})$, dilepton, 13 TeV & 1 & \textit{0.962} & \textit{0.962} & \textit{0.962} & 0.312 & 0.447 & 0.347  \\
    CMS $\sigma(t\bar{t}b\bar{b})$, $\ell+$jets, 13 TeV & 1 & \textit{0.900} & \textit{0.900} & \textit{0.900} & 0.135 & 0.269 & 0.167  \\
    \midrule
   {\bf Total associated $t\bar{t}$}  & {\bf 26}  &  {\bf 1.255 } &  {\bf 1.255 } & {\bf 1.246 } & {\bf 0.925 } & {\bf 0.888 } & {\bf 0.913 } \\
%     \midrule
%     \midrule
%   {\bf Total top}  & {\bf 260}  &   &    \\
%     \midrule
%     \midrule
%     {\bf Grand total across all non-top \& top data}   &  {\bf 4022} & 1.1623  & 1.1627  \\
 \bottomrule
\end{tabular}
\end{center}
  \caption{\small \label{tab:chi2-top}
    Same as Table~\ref{tab:chi2-baseline} now
    for the  inclusive and associated $t\bar{t}$ production datasets.
     Values in italics indicate datasets 
    that do not enter the corresponding SM-PDF fit: for those processes,
    we evaluate a posteriori the physical observables and the associated
    $\chi^2$ values using the resulting PDFs from the fit.
    For instance, top data is removed from the \nnpdfnotop,
    and for some top quark observables like $t\bar{t}t\bar{t}$ their
    PDF dependence is neglected.
      The last row indicates the total values adding together the non-top
    and top data contributions to the $\chi^2$.
}
\end{table}
%%%%%%%%%%%%%%%%%%%%%%%%%%%%%%%%%%%%%%%%%%%%%%%%%%%%%%%%%%%%%%%%%%%%%%%%%%
%%%%%%%%%%%%%%%%%%%%%%%%%%%%%%%%%%%%%%%%%%%%%%%%%%%%%%%%%%%%%%%%%%%%%%%%%%%%%%%%
