# Supplementary material for: Precision phenomenology of the PDF-BSM interplay
Source: arXiv:2503.02827 source file (2025-03-04)
Supplement: Supplementary file 30 [file table-input-dataset-top1b.tex]

%%%%%%%%%%%%%%%%%%%%%%%%%%%%%%%%%%%%%%%%%%%%%%%%%%%%%%%%%%%%%%%%%%%%%%%%%%%%%%%%%%%%%%%
\begin{table}[h!]
  \begin{center}
{\fontsize{8pt}{8pt}\selectfont
%\begin{table}[t]
  \centering
   
   \setlength{\tabcolsep}{2pt}
   \begin{tabular}{lcccccc|c|c}
     \toprule \textbf{Experiment}     & $\bf{\sqrt{s}}$\textbf{(TeV)}
     & \textbf{Channel}  &  \textbf{Observable} & $\mathcal{L}$ (fb${}^{-1}$) & $\mathbf{n_{\rm dat}}$ & \textbf{Ref.}   &\textbf{New (PDF fits)}
    &  \textbf{New (SMEFT fits)} \\
    \toprule
      \multirow{2}{*}{ATLAS}
      & 8
      & dilepton
      & $A_C$
      & $20.3$
      & 1
      & \cite{Aad:2016ove}
      & $\checkmark$                                                                     
      &  \\
%-------------------------------------------------------------------------------
      & 13
      & $\ell+$jets
      & $A_C$
      & $139$
      & 5
      & \cite{ATLAS:2022waa}
      & $\checkmark$                                                                     
      & $\checkmark$   \\
%-------------------------------------------------------------------------------
     \midrule
      \multirow{2}{*}{CMS}
      & 8
      & dilepton
      & $A_C$
      & $19.5$
      & 3
      & \cite{Khachatryan:2016ysn}
      & $\checkmark$                                                                     
      &  \\
%-------------------------------------------------------------------------------
      & 13
      & $\ell+$jets
      & $A_C$
      & $138$
      & 3
      & \cite{CMS-PAS-TOP-21-014}
      & $\checkmark$                                                                     
      &  \\
%-------------------------------------------------------------------------------
\midrule
      ATLAS/CMS comb.
      & 8
      & $\ell+$jets
      & $A_C$
      & $20$
      & 6
      & \cite{Sirunyan:2017lvd}
      & $\checkmark$                                                                     
      &  \\
\bottomrule
   \end{tabular}
   \vspace{0.3cm}
   \caption{\small Same as Table~\ref{tab:input_datasets_toppair} for the $t\bar{t}$
     asymmetry datasets.
   \label{tab:input_datasets_topasymmetries} \label{tab:asymmetries}
}
}
\end{center}
\end{table}
%%%%%%%%%%%%%%%%%%%%%%%%%%%%%%%%%%%%%%%%%%%%%%%%%%%%%%%%%%%%%%%%%%%%%%%%%%%%%%%%
