# Supplementary material for: Precision phenomenology of the PDF-BSM interplay
Source: arXiv:2503.02827 source file (2025-03-04)
Supplement: Supplementary file 36 [file table-input-dataset-top4b.tex]

\begin{table}[h!]
{\fontsize{7pt}{7pt}\selectfont
%\begin{table}[t]
  \centering
   
   \setlength{\tabcolsep}{5pt}
   \begin{tabular}{lcccc|c}
     \toprule \textbf{Experiment}     & $\bf{\sqrt{s}}$\textbf{(TeV)}
     &  \textbf{Observable} & $\mathbf{n_{\rm dat}}$ & \textbf{Ref.}   
    &  \textbf{New (SMEFT fits)} \\
    \toprule
      ATLAS
      & 13
      & $\sigma_{\text{fid}}(tl^+l^-q)$
      & 1
      & \cite{Aad:2020wog}
      & \\
%-------------------------------------------------------------------------------
     \midrule
      CMS
      & 13
      & $\sigma_{\text{fid}}(tl^+l^-q)$
      & 1
      & \cite{Sirunyan:2018zgs}
      & \\
%-------------------------------------------------------------------------------
      & 
      & $d\sigma_{\text{fid}}(tZq)/dp_T(Z)$ or $d\sigma_{\text{fid}}(tZq)/dp_T(t)$
      & 4 or 3
      & \cite{CMS:2021rvz}
      & $\checkmark$\\
\bottomrule
  \end{tabular}
  \caption{\small Same as Table~\ref{tab:input_datasets_toppair} for all the single-top production in association with a $Z$-boson included in this analysis.
     \label{tab:input_datasets_4b}
}
}
\end{table}
%%%%%%%%%%%%%%%%%%%%%%%%%%%%%%%%%%%%%%%%%%%%%%%%%%%%%%%%%%%%%%%%%%%%%%%%%%%%%%%%%%%%%%%%%%%%%%%%%%%%
