# Supplementary material for: Precision phenomenology of the PDF-BSM interplay
Source: arXiv:2503.02827 source file (2025-03-04)
Supplement: Supplementary file 37 [file 21Appendix.tex]

\appendix
\chapter{Extra Information}
Some more text ...
